# Supplementary material for: SurfFlow: high-throughput surface energy calculations for arbitrary crystals
Source: arXiv:2311.03163 ancillary file (2023-11-06)
Supplement: Supplementary file 1 [file sm.pdf]

# Supplementary Material for SurfFlow: high-throughput surface energy calculations for arbitrary crystals

Firat Yalcin, Michael Wolloch

November 6, 2023

## S1 List of considered systems

In table S1 we list the 36 diverse materials we used to test SurfFlow and especially the prediction of surface energies using bond valence sums. All structures were queried from the Materials Project. For most of those materials, we calculated the energy for all non-polar surfaces up to a maximum Miller index (MMI) of 3. For a few cases, MoP (mp-219), $AlCuPt_2$ (mp-12550), WC (mp-1894), TiS (mp-101802), and ZrTe (mp-1539), only 4 unique non-polar surfaces exist for MMI $\leq 3$, for which we added also all polar surfaces of MMI $\leq 2$, although a larger percentage of those failed due to bad convergence (as is expected for less stable surfaces).

Not included in the table are the benchmark materials anatase and rutile $TiO_2$, with MPIDs mp-390 and mp-2657.

Of a total of 928 surfaces generated for these 36 materials, 75 (8%) slabs were excluded because they had more than 100 sites. 62 of them had MMI = 3, while the other 13 had MMI = 2. Of the remaining 853, 181 (21%) were filtered out because they were polar (and not belonging to the five specific systems mentioned before). On the other hand, we had 70 polar surfaces already calculated before deciding to generally exclude polar ones and decided to include them since all the other settings were correct. Thus, we actually started calculations on 742 surfaces, 89 (12%) of which could not complete the workflow due to unrecoverable errors in one or more of the necessary DFT calculations. This failure rate is entirely acceptable for high-throughput computations but could be lowered by having an expert user look at the failed calculations and adapting the input settings through the web portal (see section S7. The resulting 653 surface energies can be found at the end of this SM in table 5. 44% of the considered slabs are asymmetric and thus have two distinct surface energies. This is a considerable proportion and highlights the need for a tool to handle asymmetric setups.

| ID | Formula | Bandgap (eV) | $E_{hull}$ (eV) | Magnetic | Space group |
|---|---|---|---|---|---|
| mp-1018028 | TiS | 0.000 | 0.000 | False | 187 |
| mp-102 | Co | 0.000 | 0.016 | True | 225 |
| mp-10905 | Al3Pt2 | 0.000 | 0.000 | False | 164 |
| mp-1138 | LiF | 8.696 | 0.000 | False | 225 |
| mp-11807 | LiPt | 0.000 | 0.000 | False | 187 |
| mp-12550 | AlCuPt2 | 0.000 | 0.000 | False | 123 |
| mp-129 | Mo | 0.000 | 0.000 | False | 229 |
| mp-13 | Fe | 0.000 | 0.000 | True | 229 |
| mp-13136 | WC | 0.000 | 0.448 | False | 225 |
| mp-135 | Li | 0.000 | 0.005 | False | 229 |
| mp-136 | Fe | 0.000 | 0.098 | False | 194 |
| mp-1487 | AlNi | 0.000 | 0.000 | False | 221 |
| mp-1502 | Al2Pt | 0.000 | 0.000 | False | 225 |
| mp-1539 | ZrTe | 0.000 | 0.000 | False | 187 |
| mp-1894 | WC | 0.000 | 0.000 | False | 187 |
| mp-1953 | TiAl | 0.000 | 0.000 | False | 123 |
| mp-2133 | ZnO | 0.723 | 0.000 | False | 186 |
| mp-219 | MoP | 0.000 | 0.000 | False | 187 |
| mp-2213 | FeNi | 0.000 | 0.000 | True | 123 |
| mp-2260 | FePt | 0.000 | 0.000 | True | 123 |
| mp-22862 | NaCl | 5.004 | 0.000 | False | 225 |
| mp-23 | Ni | 0.000 | 0.000 | True | 225 |
| mp-23193 | KCl | 5.027 | 0.000 | False | 225 |
| mp-2379 | CoSi2 | 0.000 | 0.000 | False | 225 |
| mp-2744 | LiPd | 0.000 | 0.000 | False | 187 |
| mp-2746 | MoC | 0.000 | 0.298 | False | 225 |
| mp-284 | AlCo | 0.000 | 0.000 | False | 221 |
| mp-463 | KF | 5.949 | 0.000 | False | 225 |
| mp-492 | TiN | 0.000 | 0.000 | False | 225 |
| mp-522 | CuAu | 0.000 | 0.000 | False | 123 |
| mp-579 | CrC | 0.000 | 0.254 | True | 225 |
| mp-631 | TiC | 0.000 | 0.000 | False | 225 |
| mp-66 | C | 4.114 | 0.138 | False | 227 |
| mp-91 | W | 0.000 | 0.000 | False | 229 |
| mp-930 | ZrP | 0.000 | 0.043 | False | 225 |
| mp-987 | ZnCu | 0.000 | 0.000 | False | 221 |

Table 1: List of materials used to test SurfFlow and evaluate the performance of the bond valence sum predictions to the surface energies.

## S2 Surface energy calculation scheme for a symmetric nonstoichiometric slab

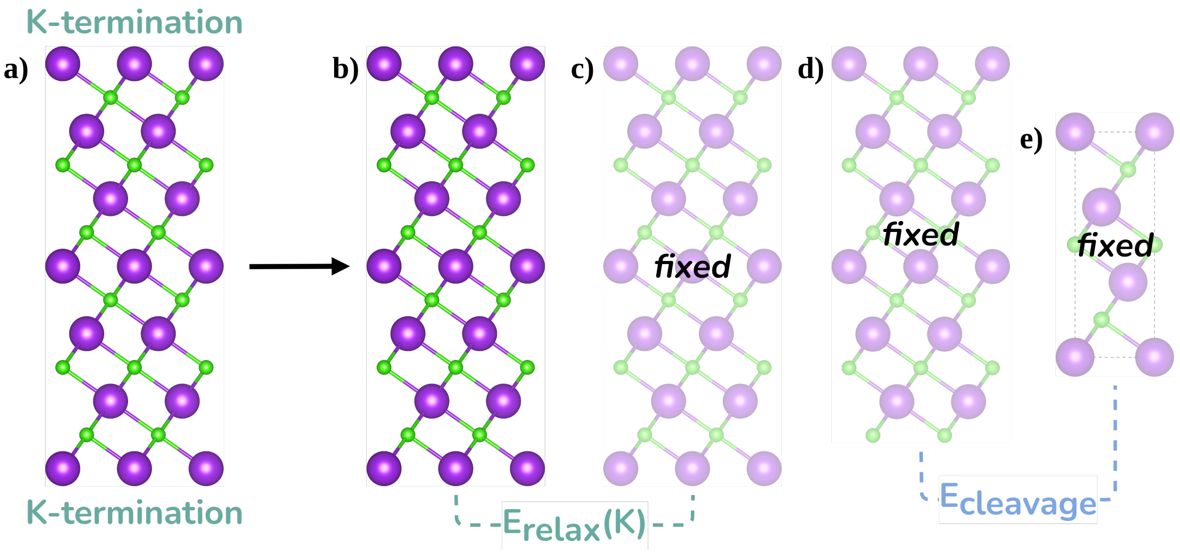


Figure 1: Surface energy calculation scheme for a symmetric KCl (mp-23193) 111 slab with K terminations. In order to calculate the surface energy of the slab (a), we need the energies of (b) relaxed symmetric slab, (c) static symmetric slab, (d) stoichiometric static slab with complementary K and Cl terminations, and (e) the oriented unit cell.

In the main paper, we highlighted the surface energy calculation scheme for an asymmetric and stoichiometric slab, emphasizing that this type of surface is always possible to generate and deal with using the method by Tian and coworkers [1].

This method, however, can be just as easily applied to the case of a symmetric and nonstoichiometric slab. In this case, the relaxation energies for the top and the bottom terminations are equal, since the slab is symmetric, and can be readily calculated from a fully relaxed slab and a static slab.

$$E_{slab}^{relax}(T) = \frac{1}{2A}\left[E_{slab}^{relaxed} - E_{slab}^{static}\right] \quad , \tag{1}$$

The cleavage energy, on the other hand, is slightly trickier to calculate since we have a nonstoichiometric system on our hands. The approach here is to generate an additional, asymmetric and stoichiometric slab with the same top termination as the original slab, and use it to calculate the cleavage energy as we do for the asymmetric stoichiometric case.

$$E_{cleavage}(T) = \frac{1}{2A}\left[E_{sto.slab}^{unrelax} - NE_{bulk}\right] \quad , \tag{2}$$

where $E_{sto.slab}^{unrelax}$ is the total unrelaxed energy of the asymmetric and stoichiometric slab.

This scheme is schematically shown in Fig. 1.

## S3 Polar surfaces

A polar surface refers to a surface of a material where the termination or arrangement of atoms leads to a non-zero net electric dipole moment in the direction of the surface normal. If uncompensated, this results in a divergent surface energy as the number of layers of the slab increases [2].

Such surfaces usually undergo substantial, energetically unfavorable changes to compensate for their polarity. These can include changes in the surface geometry, stoichiometry, or electronic structure. Regardless of these compensation mechanisms, however, polar surfaces tend to have larger surface energies compared to non-polar facets of the same material.

In our workflow, we have decided to try and filter out any polar surfaces that we encounter by default. This is achieved by guessing ionic charges based on oxidation states via pymatgen for each slab and then proceeding only with slabs that do not show polarity [3].

However, a crystal might have very few non-polar surfaces (see section S1), or a user might want to compute the surface energies of polar slabs for another reason, so we strive to make this as accurate as possible.

To this end, we include dipole corrections to the energy, the potential, and the forces in our VASP calculations for polar systems along the out-of-plane lattice vector. This is necessary to correct for erroneous contribution from the dipole moments of the periodic images to the total energy, forces, and potential and allows for the evaluation of the work function for polar surfaces. However, calculations containing the corrections are much tougher to converge. To overcome this issue, we use a two-step procedure in our relaxation subworkflows that is only used if a slab is polar: In the first step, we perform a non-corrected pre-calculation to extract the wavefunctions, which we then use in the dipole corrected calculation for easier convergence. We should also note that the dipole correction scheme in VASP is limited to systems where the direction in which the correction is to be applied (third lattice vector in our case, where the vacuum region is added) is orthogonal to the other two lattice vectors, i.e. $\alpha = \beta = 90°$.

Polar surfaces are generally quite complex to describe correctly in a periodic model system. In order for a polar surface to be stable, it has to undergo a polarity compensation mechanism in order to cancel out the thickness dependence of the dipole moment contributions from the charged layers in order to avoid divergent surface energies [4, 5, 6]. This can happen in several different ways: E.g. through induced surface charges as a result of partially-filled surface states; changes in the surface composition; through adatoms/vacancies; or others [5]. One should note that they are different from the dipole corrections applied in VASP described above, where the dipole moment that is corrected is usually the leftover dipole moment after polarity compensation occurs through one or more of the mechanisms mentioned.

Reconstructed polar surfaces tend to have lower surface energies than those that only rearrange electronically, but are difficult to model, especially in a high-throughput framework (see section S6). Therefore, we advise users to be cautious with polar surfaces and check the results very carefully against experimental data if possible.

## S4 Note on cleavage energies and electronegativities

In the surface energy calculation method [1] we employ in this workflow, it is assumed that the cleavage energies are equal for complementary terminations. In the study where the method is presented, they note that this assumption is valid only because the electronegativities $\chi$ of Mo and P are equal. We understand the argument to mean that if this requirement is not satisfied, charges on the surface would be different in a truly cleaved surface than in the slab model, where they are the nominal atomic charges. While this highlights difficulties with polar slabs (which we discuss in section S3), we do not quite see how this affects the assumption that the cleavage energy is distributed equally between the complementary surfaces. The cleavage energy is the energy of the broken bonds, and while it might differ depending on the final electronic state, its distribution is an unrelated matter, and, in our opinion, more a question of definition.

To analyze this question further, we apply another approach to calculating cleavage energies, which does not claim to be restricted to closely matching electronegativities. Heifets et al. [7] have shown that given an asymmetric surface with terminations $T_1$ and $T_2$, energies of two symmetric and non-stoichiometric slabs, having terminations $T_1$ and $T_2$, can be used to calculate cleavage energies of the two terminations. We performed some calculations to see the effect of electronegativity differences in cleavage energies in binary materials comparing these two methods.

From Fig. 2, we see that only when the electronegativity difference is greater than $\sim 2.0$ we start seeing noticeable differences between the two approaches to compute cleavage energy from Tian and Heifets, respectively.

Heifets approach, however, suffers from the same drawbacks of generating symmetric slabs in general, which is that it is not always possible with all required symmetries (inversion, mirror, or screw axis). For instance, for the materials given in Fig. 2 and a maximum Miller index of 2, only 20 (of which we report 17 due to convergence issues with the remaining 3) out of a total possible 157

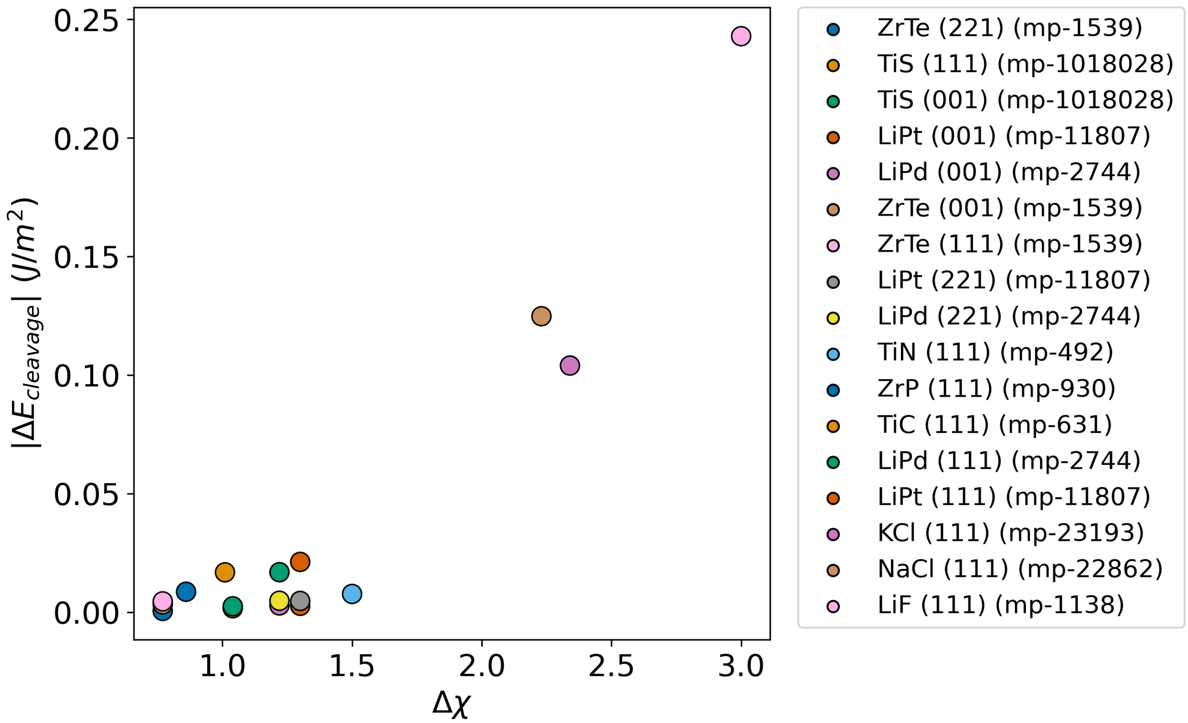


Figure 2: Absolute difference in cleavage energies between the method by Tian et al. [1] and the method by Heifets et al. [7] with respect to the difference in electronegativities $\Delta\chi$ of the constituent species.

asymmetric surfaces could be modified to be symmetric, which is a requirement for the method by Heifets et al.

This highlights the big drawback of this method compared to the one we decided to employ, and why in the end it was not suitable for our high-throughput workflow.

We nevertheless caution the user to be extremely cautious when calculating surface energies for binary systems with large ($>2.0$) electronegativity differences. While we believe that the assumption of equal distribution of cleavage energy still holds, we concede, based on the presented data, that the error in cleavage energy will become significant. We also note that the method we employ in calculating cleavage energies results in smaller values compared to the method by Heifets et al. (all the points in Fig. 2 lie below $y = 0$ when we don't look at absolute differences), and as a result, the calculated surface energies will be smaller in the end.

# S5 Workflow structure and subworkflows

In Fig. 3 we show a flowchart of the whole SurfFlow workflow, from reading inputs to calculating the Wulff shape for all N unique Miller indices (hkl) and all M unique surface terminations for each of those. The boxes marked with numbers refer to a subworkflow or an independent step. The generation of reference structures and selection of calculation types to determine which steps need to be taken for each combination of stoichiometry and symmetry (step 3) and the according calculation of the surface energy (step 4) are discussed in detail in the main paper. Furthermore, we explain the input selection and the default parameters in subsection S5.1, and the slab optimization in subsection S5.2 of this SM.

## S5.1 Read Inputs

The workflow starts with the user defining some input parameters, either via a command line tool, a .yaml file, or the web app (see section S7). These parameters can be grouped into four categories; computational, slab generation, bond valence sum (BVS) filtering, and database. Computational parameters (Table 2) consist of important quantities used in the DFT calculation such as the energy

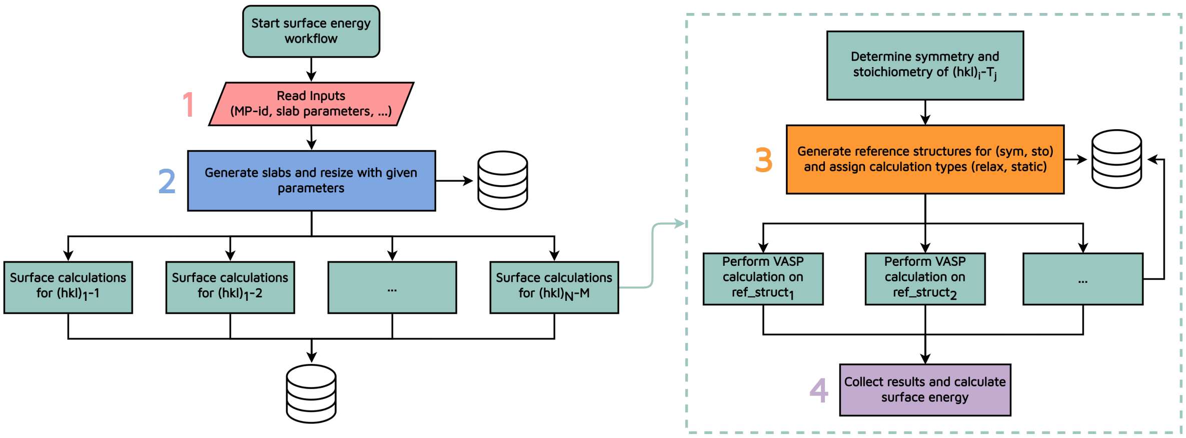


Figure 3: Flowchart of the whole workflow, determining surface energies and Wulff shape for a single material.

cutoff for plane waves, the density of points for the k-mesh generation to sample the Brillouin zone, and the exchange-correlation functional used. Slab generation parameters (Table 3) deal with the geometry of the slabs generated and can affect the system sizes and terminations. BVS filtering parameters (Table 4) handle the prescreening process for low-energy surfaces. Finally, the database parameters define where in the database to query from and write into. Note that slabs that are not selected for DFT calculations by the prescreening are not added to the database.

| **Parameter** | **Type** | **Default** | **Description** |
|---|---|---|---|
| use_vdw | boolean / string | False | Flag to use van der Waals interactions |
| functional | string | "PBE" | Exchange correlation functional to use |
| use_spin | boolean | True | Flag to perform spin-polarized calculations |
| encut | integer | 400 | Plane wave energy cutoff [eV] |
| k_dens | float | 5.00 | K-point density used in generating the k-mesh grid [1/Å] |
| is_metal | boolean | None [1] | Flag to indicate if the system is metallic |

Table 2: Computational parameters related to the VASP calculations.

## S5.2 Resizing slabs

Most of the slab generation is handled by pymatgen. First, an oriented unit cell (OUC) for a given Miller index is generated by applying the necessary transformations to the conventional bulk unit cell so that the Miller direction is aligned with the $c$-direction [8]. The OUC is then replicated along $c$, where the number of replications is determined by the `min_slab_size` parameter of pymatgen. Here, two issues may arise, that do not lead to optimal results. First, since the only criterion is the number of layers, the resulting slab might be too thin depending on how close the layers are together. The second issue arises with high-index surfaces of some materials when one also requires the slabs to be as orthogonal (referring to the mutual orthogonality of the three lattice vectors) as possible. In this case, the OUC may end up becoming very large, consisting of a large number of layers, and since the smallest slab pymatgen can generate contains at least one OUC, the resulting system is far from ideal for high-throughput work.

In order to optimize these troublesome systems, we implemented an additional method that allows for precise resizing of slabs by removing layers from the bottom until a user-defined criterion is met. At this point, the definition of an atomic layer becomes important. We define an atomic layer by grouping up atomic sites with respect to the third component (vacuum is always assumed to be in the

[1] This flag determines some of the VASP input parameters such as the smearing method. Since the metallic character of a surface may differ from that of the bulk, we leave this parameter to the user. If left empty, the bandgap of the bulk structure is used to determine the metallicity.

| Parameter | Type | Default | Description |
|---|---|---|---|
| symmetrize | boolean | False | Flag to symmetrize the slabs generated |
| slab_thick | integer | 8 | Thickness of the slab in number of layers (num. layers) |
| vac_thick | float | 30.00 | Thickness of the vacuum [Å] |
| primitive | boolean | True | Try to find primitive cell vectors normal to the surface |
| lll_reduce | boolean | True | Whether or not the slabs will be orthogonalized |
| layer_tol | float | 0.05 | How far apart atoms may be to belong to one layer [Å] |
| max_normal_search | string / integer | "max" | Parameter related to search for orthogonal cells |
| resize | boolean | True | Flag to enable slab resizing (see section S5.2) |
| preserve_terminations | boolean | True | Flag to enable termination preservation (see section S5.2) |
| slab_thick_A | float | 10.00 | Minimum thickness of the generated slabs [Å] |
| minimize_structures | boolean | False | Force smallest slabs possible (may reduce accuracy) |
| match_ouc_lattice | boolean | True | Force OUC lateral cell for slabs (may increase size) |
| calculate_bonds | boolean | True | Flag to enable calculation of broken bonds |
| center_slab | boolean | True | Center the slab in the unit cell |
| max_nsites | integer | 100 | Maximum number of sites in a slab |
| filter_polar | boolean | True | Whether to filter out polar slabs |

Table 3: Parameters used in slab generation.

| electronically **Paremeter** | Type | Default | Description |
|---|---|---|---|
| bvs_min_N | integer | 10 | Number of surfaces to calculate |
| bvs_min_N_hkl | integer | 1 | Number of surfaces to calculate for each unique Miller index |

Table 4: Parameters used in BVS filtering.

third lattice vector direction) of their fractional coordinates, which we will call the c-coordinate from now on. We allow the user to set a tolerance parameter, `layer_tol`, so that sites with c-coordinate values that are within this tolerance with each other are assumed to constitute a layer. Once layers are defined, we can proceed with the removal of layers until the desired thickness is reached.

The process of removing the layers is not as straightforward as it first appears to be, however, since the assumption that the cleavage energies are split evenly among two terminations only applies when the two terminations are complementary, and arbitrarily removing layers may (and in most cases does) lead to a different termination than the one we started with. In order to overcome this problem and preserve terminations during resizing, we instead group all the sites within a region of thickness $d_{hkl}$, the distance between consecutive Miller planes with identical termination, together. Since all the planes belonging to a family denoted by hkl are equivalent to each other by the symmetry of the lattice, removing a chunk with $d_{hkl}$ thickness doesn't alter the bottom termination, ensuring that our approach of calculating surface energies using cleavage energies remains applicable.

The final size of the slab is defined by the user through two parameters, `slab_thick` and `slab_thick_A`. The former, `slab_thick`, is the number of layers that the user wants in the final slab, and the latter, `slab_thick_A` is the minimum thickness for the final slab in Angstroms. The resizing process by removing layers from the bottom proceeds until we arrive at the smallest slab that satisfies both criteria.

The resizing process is outlined for KCl (332) in Fig. 4. We start with the smallest slab pymatgen generated (a) for this material with our default slab generation parameters containing 88 atomic sites clustered to 44 atomic layers. We then identify Miller planes of $d_{hkl}$ thicknesses, among which we choose a cutoff plane that is consistent with the slab thickness parameters (at least 8 layers and at least 10 Å). As the last step, all layers below (excluding) the cutoff plane are removed (c), leaving us with a much more manageable slab with the original terminations preserved.

Note that by default we set the pymatgen parameter `max_normal_search` to the maximum absolute value of the individual indices for the Miller index of a given surface to generate slabs as orthogonal as possible. This is because dipole corrections to the potential and forces in VASP are only possible for orthorhombic cells, and it is recommended to at least have the direction in which corrections will be applied be orthogonal to the other two directions. This setting increases the size of the oriented

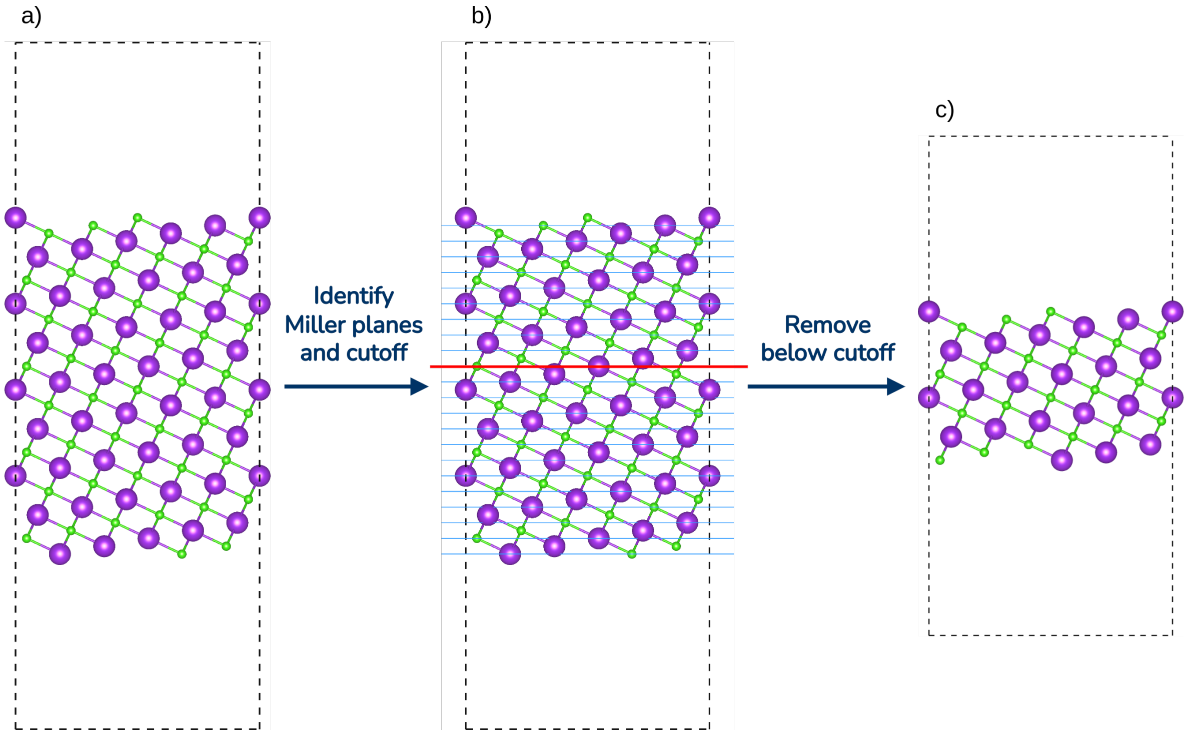


Figure 4: (color online) Step-by-step slab resizing procedure. Starting with the smallest slab generated (a), Miller planes and cutoff plane are identified (b), and layers below the cutoff (excluding) are removed (c).

unit cell, making the resizing step necessary for polar surfaces even if the user decides to forego the resizing with a smaller `max_normal_search`.

## S6 Note on reconstructions

When a surface is created from a bulk, the missing bonds lead to relaxations and possibly also reconstructions. In contrast to relaxations, reconstructions alter the symmetry of the surface. While reconstructions can preserve the total number of atoms per layer (conservative reconstruction), this is not always the case (non-conservative reconstruction), Additionally, adatoms might absorb, or vacancies can be formed while atoms or molecules desorbed to lower the surface energy depending on the surface and the environmental conditions.

For monoatomic crystals, Tran et *al.* [9] have calculated known reconstructions of several crystals like Si-diamond (100), (110) and (111), fcc-Au (110), among others. In total 12 different reconstructions are available to date, eight for fcc (110 and 111), three for diamond (100, 110, and 111), and one for bcc (100) surfaces.

For more complex systems, the situation can become nearly arbitrarily complex, and tabulating reconstructions is no longer feasible. Without experimental information, crucial parameters such as the size of the supercell needed to accommodate the reconstruction, and the presence of adatoms or vacancies required are unknown. Thus, the search space for unknown surface reconstructions is significant in size. For instance, Mora-Fonz et al. [10] studied stable configurations of ZnO (0001) where they probed more than 500,000 structures in total to find the most likely reconstructions.

Experimental techniques like low-energy electron diffraction (LEED), Rutherford backscattering spectroscopy, and most of all scanning tunneling microscopy (STM) can indicate supercell size and provide other information on reconstruction, but chemical intuition and model calculations are usually still needed to nail down the exact structure.

Even if experimental data are available, a manual search for reconstructions is usually only practical for very simple systems. Several approaches based on genetic algorithms [11, 12, 13] have been used in the last decade to find surface reconstructions [14, 15, 16, 17, 18, 19].

Very recently, the machine learning and graph-theory assisted universal structure searcher (MAGUS) framework has been employed to search for surface reconstructions [20].

It should be clear from these paragraphs that an exhaustive treatment of reconstructions is a daunting task and far beyond the scope of this paper. For these reasons, we do not make any deliberate attempt to search for reconstructions in our workflow.

# S7 Web application for workflow control

We provide a user-friendly web application (Fig. 5) to submit and control workflows easily instead of going through Python scripts in case of submission, or the `launchpad` command-line tool provided by `FireWorks` in case of workflow monitoring. The submission panel (a) allows one to modify all the possible parameters in the system, from computational to slab generation, while also allowing one to set custom INCAR parameters for specific systems.

The workflow panel (b), apart from providing a simple overview of the workflows on the launchpad, also allows users to access more detailed information about the specific `fireworks` within a workflow. In case there are failed ("fizzled" in `FireWorks` lingo) `fireworks`, the user can query for such fireworks and access the cause of the error. Additionally, the "fizzled" fireworks can be resubmitted with user-defined calculation parameters (INCAR) right from the application itself. This web application minimizes the need for an active terminal and was the main entry point that the authors used to submit workflows and check on their progress.

It is also possible to query, from the web application, currently available surface energies in the database using either the Materials Project ID of a material or a more general MongoDB query string (equivalent would be {"mpid": "mp-XX"}). This query returns an interactive table of surface energies and calculation details for each. The user can then ask for a Wulff shape to be generated with these surface energies, upon which an interactive Wulff shape is generated with the help of pymatgen.

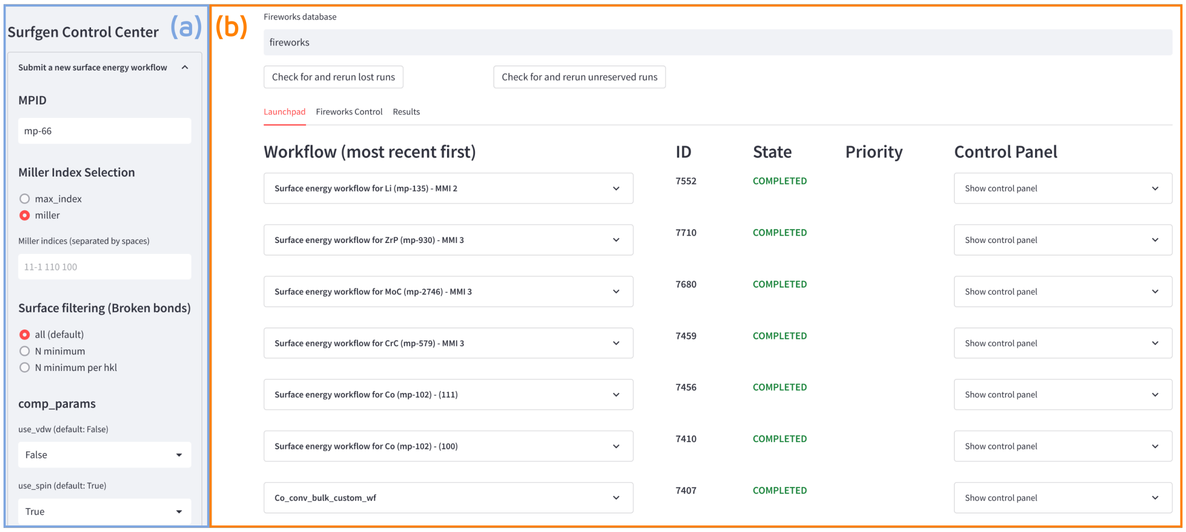


Figure 5: (color online) An overview of the web application, with the submission panel (a), and the workflow overview and controls (b).

# S8 On the choice of functional and pseudopotentials

The data presented in this paper were calculated with the PBE functional, which is still the de-facto standard for DFT calculations [21]. The main reason for this choice is the usage of bulk structures from the Material Project, which are optimized with the PBE functional. Note that both PBE and LDA [22] have been shown to produce reasonable surface energies, but PBE underestimates surface energies for systems with large correlation energy [23]. Patra et al. compared several common den-

sity functionals and showed that SCAN+rVV10 shows the lowest mean absolute percentage errors concerning experimental data for low index, monoatomic, and metal surfaces [24].

We use PBE+U if U values are defined in the bulk structure queried from the Materials Project to better handle correlation effects without exploding computational cost. We also implemented optimized input sets and slightly adapted workflows for LDA and the SCAN functional [25] (using the SCAN specific vasp input sets and atomate fireworks [26]), as well as van der Waals corrections of choice, so e.g. SCAN+rVV10 might be used without any added complexity by just setting `functional = SCAN` and `use_vdw = rVV10` in the inputs.

We use the VASP `potpaw_PBE.54` PAW pseudopotenial set for all calculations in this work, and the code also selects this set for SCAN calculations. If LDA is selected as a functional, the `potpaw_LDA.54` set will be used instead. Since there are several options for most elements in the periodic table, a mapping must be chosen to unambiguously define the pseudopotentials to be used. We default to the mapping of the MPRelaxSet, but the user is able to adjust the mapping via the input dictionary, or by adding a different mapping to the defaults.json file.

# S9 Caching system

The `tasks` collection of the Fireworks database contains an entry for each successful VASP calculation. These entries contain detailed information about calculations such as the inputs, outputs, calculation folders, and runtime statistics. Each entry also contains a `task_label` field which can be defined when initializing the python object (Firetask) attached to the VASP calculation. This allows for convenient querying of the tasks collection for calculations. For each VASP calculation that we define in the workflow, we generate a unique ID based on the input parameters and the structure and attach this ID to the calculation as its `task_label`. This ID is also attached to the high-level database entries for that particular surface energy calculation. During the main workflow, whenever a VASP sub-workflow runs, two checks are performed to see if this calculation has already been performed before. First, the high-level database is queried with this unique ID to check if it already contains the parsed outputs. If so, the sub-workflow ends here. If not, the same check is performed for the low-level database. If a task with the unique ID as its `task_label` is found, the entry is parsed and moved to the high-level database, and the VASP calculation is not performed. Finally, if the unique ID is not found in either of the databases, the workflow proceeds with the VASP calculation, at the end of which there will be entries in both databases for the calculation.

Our caching system allows us to optimize performance by avoiding unnecessary duplicate calculations and storing frequently used results. This can be particularly useful in situations where a calculation needs to be performed multiple times, such as when determining the energy of an oriented bulk structure for different terminations of a single Miller index, for which only a single VASP calculation suffices. Additionally, the caching system makes it more efficient to run the workflow on a shared database, where different users can run the workflow without worrying about duplicates.

# S10 Comparison of monoatomic crystals to the Materials Project / Crystalium

To test our automatic workflows, our choice of parameters, and the bond valence sum approximation to the surface energy, we have also calculated a few elemental crystals and have compared them to the Materials Project data from Tran and coworkers [9]. In Fig. 6 we see that for most materials the results are nearly identical, which is not too surprising, given that the same functional and similar computational parameters have been used. Significant deviations are however observed for 7 Co surfaces, as well as the 211 surface of Mo and the 310 surface of Fe, for all of which we observe significantly lower surface energies.

To explain these deviations, we have looked at other literature values to compare our, and the Material Project's, results. For Fe (310), our value seems to be confirmed by other previous works [27, 28, 29]. For Mo (211), we also find data supporting our result, that the facet should be exposed in the Wulff shape [30, 31]. We assume that those two calculations had some convergence issues or other problems in Ref. [9], which are bound to happen from time to time in large-scale high-throughput DFT studies.

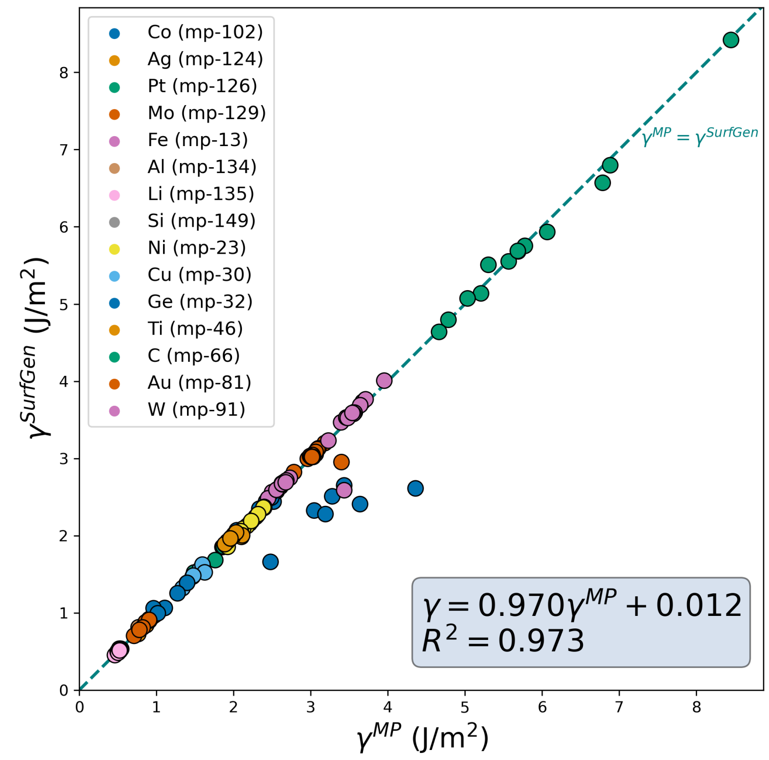


Figure 6: Comparison of SurfFlow result of elemental crystals with data from the Materials Project [9].

Especially for the case of cobalt, where we found recent calculations by Lin et *al.* [32] a more detailed discussion is needed because there are systematic deviations for more than one surface facet. We repeated our workflow with a different pseudo-potential that moves the $3p$ states from the frozen core to the valence states to have potentially more accurate results. The results are plotted in Fig. 7.

We clearly see that the computed data from both our pseudopotential matches the results of reference [32] very well, while some surfaces deviate significantly for the Materials Project data. We attribute these deviations to an old pseudopotential file that was used by Tran et *al.* [9]. Their POTCAR, `PAW_PBE Co 06Sep2000`, is from the 91 set of potentials which are deprecated and no longer recommended. We use the same type of potential (PAW, PBE, only $3d$ and $4s$ states as valence), but a newer version of it, that belongs to the recommended 54 set, `PAW_PBE Co 02Aug2007`. The data was confirmed using the `PAW_PBE Co_pv 23Apr2009` potential from the same set.

# S11 Analysis of the few materials with very bad correlation between bond valence sum and surface energy

As mentioned in the main paper, we have some systems with very bad correlation between the BVS-estimated, and the computed surface energy. Those are bcc Li (mp-135, $r = -0.087$), $\gamma$-TiAl (mp-1953, $r = -0.070$), and, to a lesser extent, bcc and hcp Fe (mp-13, $r = 0.573$; mp-136, $r = 0.550$)

## S11.1 bcc and hcp Fe

Schönecker and coworkers computed the surface free energy of the (100) and (110) facets of bcc Fe, separating vibrational, electronic, and magnetic contributions to the free energy using the quasiharmonic approximation [33]. They show a modest influence of temperature on the surface energy from 0 K to $\sim$ 500 K, dropping from 2.51 J/m$^2$ to 2.35 J/m$^2$ for the (100) facet and from 2.48 J/m$^2$ to 2.3 J/m$^2$ for the (110) facet. This is very well in line with our 0 K results of 2.56 J/m$^2$ and 2.48 J/m$^2$ for the (100) and (110) facets. Upon $\sim$ 1600 K, where we are already in the high temperature $\delta$ bcc

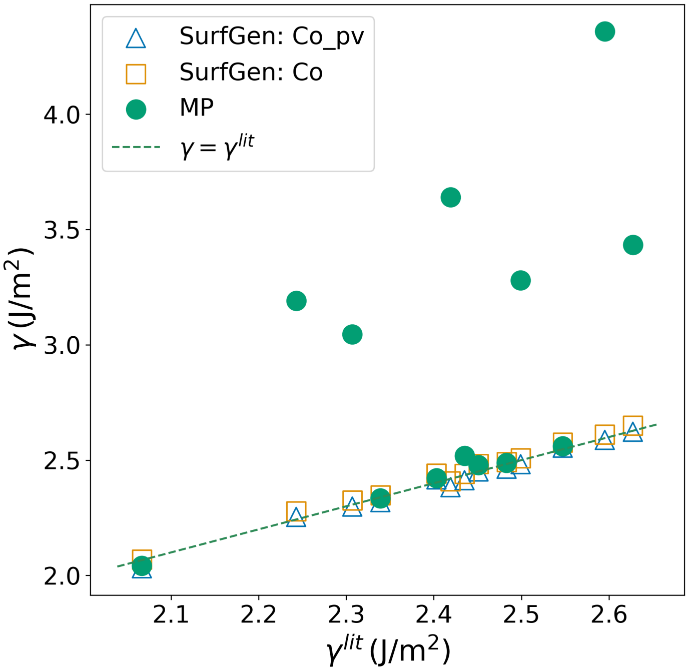


Figure 7: Comparison of SurfFlow result for Co, using two different pseudopotentials, with and without $3p$ states as valence, with the materials project (MP) [9] and recent calculations from Lin and coworkers [32], which we will treat here as the reference values $\gamma^{lit}$.

phase, they drop more considerably to about 1.82 J/m$^2$ and 1.80 J/m$^2$ for (100) and (110), respectively. This is pretty much in line with high temperature ($\sim$ 1700 K) measurements from the sixties for iron wires at 1.95±10% J/m$^2$ for $\delta$ iron [34]. Unfortunately, we were not able to find more up-to-date or low-temperature experimental data on iron surface energies.

However, these data, as well as the generally excellent agreement between our current work and the data from the Materials Project [9], lead us to believe that our computed surface energies for Fe are correct, and the BVS prediction fails for this material.

Ma et *al.* [35] report a similar low correlation between their slightly different variation of the bond valence model and their computed surface energy for both bcc and fcc Fe, blaming the complex chemistry due to the half-filled $d$-band, magnetism, and strong relaxations. Indeed, their unrelaxed bcc Fe structure has a decent correlation, although this is not true for fcc Fe. There is experimental evidence for strong relaxations (around 17% contraction in the first layer, and 10% in the second) in at least the bcc Fe(111) surface [36].

It is probable, that the partially strong relaxation effects in bcc, fcc, and hcp iron do not play well with the BVS method, which is calculated for non-relaxed slabs. Compared to Ref. [35] and our data for $\gamma$-TiAl and bcc Li, the correlation we achieve is significantly better, but nevertheless a lot worse than the median value.

## S11.2 $\gamma$-TiAl

We believe that similar factors as iron might play a role in the case of $\gamma$-TiAl, where the Ti $d$-states hybridize with the Al $p$-states just below the Fermi energy. Sang and coworkers made highly accurate charge density distribution measurements in $\gamma$-TiAl using quantitative convergent beam electron diffraction [37]. They compared their results to full electron linearized augmented plane wave calculations done with WIEN2k [38] and VASP calculations based on projector augmented waves, as we use in this work. Both methods overestimated charge density localization between Ti second nearest neighbors in addition to VASP calculations having other significant deviations from both the WIEN2k

and the experimental data. If highly accurate parameters are chosen, VASP and other plane wave pseudopotential codes achieve a very high precision compared to all-electron codes, as has been very recently shown for a large test set [39]. It also has to be considered that we consider the Ti $3p$-states as valence in our calculations, while Sang et al. did not. However, it is entirely possible that our surface energy DFT data is not correct for some or all facets of TiAl due to the discrepancies discussed in Ref.[37]. As we have seen in Fig. 7 for Co, another $3d$ metal, even errors of nearly 100% in the surface energy can occur for some facets if the potential is not ideal, resulting in bad BVS/$\gamma$-correlation.

We have compared our surface energy data for $\gamma$-TiAl with literature data. Song et al. computed surface energies of low index surfaces in 2012 using the PW91 GGA functional [40]. They also report previous calculations in their paper. One needs to be aware that the bulk cell used in their work is of fcc type containing 4 atoms, while the conventional standard structure (as defined in Ref. [41]) for $L1_0$, $\gamma$-TiAl is a tetragonally distorted bcc cell with 2 atoms. Thus the surface facets described by Song et al. are generally not equivalent to the ones we report.

For the two terminations of the 001 surface, our results 2.12 J/m$^2$ (Al) and 2.13 J/m$^2$ (Ti) agree well with the data of Ref.[40] at 2.17 and 2.18 J/m$^2$, respectively. For the 100 surface which is symmetrically equivalent to the 110 surface of Ref.[40], we find 2.02 (Al) and 2.00 J/m$^2$ (Ti) that also agree well with the values listed, 2.08 and 2.06 J/m$^2$. Finally, for the two symmetric surfaces, 101 and 110, which are symmetrically equivalent to the 111 and 100 in Ref.[40], the values we calculate at 1.69 and 1.63 J/m$^2$ are in good agreement with the values listed at 1.75 and 1.70 J/m$^2$.

However, those data also have been calculated with a pseudopotential code and we have seen from Ref.[37] that even for all-electron calculations the charge density is not entirely accurate. While we can not fully resolve the reason for the nonexisting BVS/$\gamma$-correlation for this system, we think that the $3d$-$3d$ interaction is the most likely cause of it.

### S11.3 bcc Li

Li has an extremely different chemistry than Fe and TiAl, with a single 2s valence electron, and is non-magnetic. However, compared to the other bcc metals we have calculated, both the spread in bond valence sums $\Delta_{\mathrm{bvs}}(\mathrm{Li}) =\sim 0.05$ and in the surface energies $\Delta_{\gamma}(\mathrm{Li}) =\sim 0.08\,\mathrm{J/m^2}$ are extremely small. This is due to the weak bonding in lithium, which results in low BVS and generally low surface energies (around 0.51 J/m$^2$ on average). Additionally, we see that many of the surfaces have nearly indistinguishable surface energies in this system, as we have seen also for TiAl. Another bcc metal, with more difficult chemistry but stronger bonding and larger differences in surface energy, is e.g. W (mp-91, $r = 0.959$) For comparison here $\Delta_{\mathrm{BVS}}(\mathrm{W}) =\sim 0.88$ and $\Delta_{\gamma}(\mathrm{W}) =\sim 0.776\,\mathrm{J/m^2}$ are about one order of magnitude larger.

## S12 Detailed table of results

In table 5 (after the references) we print most of the results computed in this study. In total, 36 materials were considered, 8 of them monoatomic, the rest compounds with 2 or 3 species. A compact list of these systems and some information on them can also be found in section S1 of this SM.

## References


[1] X. Tian, T. Wang, L. Fan, Y. Wang, H. Lu, Y. Mu, A DFT based method for calculating the surface energies of asymmetric MoP facets, Applied Surface Science 427 (2018) 357–362. doi:10.1016/j.apsusc.2017.08.172.
URL http://dx.doi.org/10.1016/j.apsusc.2017.08.172https://doi.org/10.1016/j.apsusc.2017.08.172

[2] P. W. Tasker, The stability of ionic crystal surfaces, Journal of Physics C: Solid State Physics 12 (22) (1979) 4977–4984. doi:10.1088/0022-3719/12/22/036.

[3] S. P. Ong, W. D. Richards, A. Jain, G. Hautier, M. Kocher, S. Cholia, D. Gunter, V. L. Chevrier, K. A. Persson, G. Ceder, Python Materials Genomics (pymatgen): A robust, open-source python library for materials analysis, Computational Materials Science 68 (2013) 314–319. doi:10.1016/

j.commatsci.2012.10.028.
URL https://www.sciencedirect.com/science/article/pii/S0927025612006295

[4] C. Noguera, Polar oxide surfaces, Journal of Physics Condensed Matter 12 (31) (2000). doi:10.1088/0953-8984/12/31/201.

[5] J. Goniakowski, F. Finocchi, C. Noguera, Polarity of oxide surfaces and nanostructures, Reports on Progress in Physics 71 (1) (2008). doi:10.1088/0034-4885/71/1/016501.

[6] C. E. Dreyer, A. Janotti, C. G. Van De Walle, Absolute surface energies of polar and nonpolar planes of GaN, Physical Review B - Condensed Matter and Materials Physics 89 (8) (2014) 1–4. doi:10.1103/PhysRevB.89.081305.

[7] E. Heifets, R. I. Eglitis, E. A. Kotomin, J. Maier, G. Borstel, *Ab Initio* modeling of surface structure for SrTiO 3 perovskite crystals, Physical Review B 64 (23) (2001) 235417. doi:10.1103/PhysRevB.64.235417.

[8] W. Sun, G. Ceder, Efficient creation and convergence of surface slabs, Surface Science 617 (2013) 53–59. doi:10.1016/j.susc.2013.05.016.
URL https://www.sciencedirect.com/science/article/pii/S003960281300160X

[9] R. Tran, Z. Xu, B. Radhakrishnan, D. Winston, W. Sun, K. A. Persson, S. P. Ong, Surface energies of elemental crystals, Scientific Data 3 (1) (2016) 160080. doi:10.1038/sdata.2016.80.
URL https://doi.org/10.1038/sdata.2016.80

[10] D. Mora-Fonz, T. Lazauskas, M. R. Farrow, C. R. A. Catlow, S. M. Woodley, A. A. Sokol, Why Are Polar Surfaces of ZnO Stable?, Chemistry of Materials 29 (12) (2017) 5306–5320. doi:10.1021/acs.chemmater.7b01487.

[11] C. W. Glass, A. R. Oganov, N. Hansen, Uspex-evolutionary crystal structure prediction, Computer Physics Communications 175 (2006) 713–720. doi:10.1016/j.cpc.2006.07.020.
URL www.elsevier.com/locate/cpc

[12] Y. Wang, J. Lv, L. Zhu, Y. Ma, Calypso: A method for crystal structure prediction, Computer Physics Communications 183 (2012) 2063–2070. doi:10.1016/j.cpc.2012.05.008.

[13] M. K. Bisbo, B. Hammer, Efficient global structure optimization with a machine-learned surrogate model, Physical Review Letters 124 (2020) 086102. doi:10.1103/PhysRevLett.124.086102.
URL https://journals.aps.org/prl/abstract/10.1103/PhysRevLett.124.086102

[14] Q. Wang, A. R. Oganov, Q. Zhu, X.-F. Zhou, New reconstructions of the (110) surface of rutile $tio_2$ predicted by an evolutionary method, Phys. Rev. Lett. 113 (2014) 266101. doi:10.1103/PhysRevLett.113.266101.
URL https://link.aps.org/doi/10.1103/PhysRevLett.113.266101

[15] S. Lu, Y. Wang, H. Liu, M. S. Miao, Y. Ma, Self-assembled ultrathin nanotubes on diamond (100) surface, Nature Communications 5 (2014) 1–6. doi:10.1038/ncomms4666.
URL www.nature.com/naturecommunications

[16] Q. Wang, A. R. Oganov, O. D. Feya, Q. Zhu, D. Ma, The unexpectedly rich reconstructions of rutile tio2(011)-(2 $\times$ 1) surface and the driving forces behind their formation: An: ab initio evolutionary study, Physical Chemistry Chemical Physics 18 (2016) 19549–19556. doi:10.1039/c6cp01203e.
URL www.rsc.org/pccp

[17] L. R. Merte, M. S. Jørgensen, K. Pussi, J. Gustafson, M. Shipilin, A. Schaefer, C. Zhang, J. Rawle, C. Nicklin, G. Thornton, R. Lindsay, B. Hammer, E. Lundgren, Structure of the sno2 (110)- (4$\times$1) surface, Physical Review Letters 119 (2017) 096102. doi:10.1103/PhysRevLett.119.096102.
URL https://journals-aps-org.uaccess.univie.ac.at/prl/abstract/10.1103/PhysRevLett.119.096102

[18] H. A. Zakaryan, A. G. Kvashnin, A. R. Oganov, Stable reconstruction of the (110) surface and its role in pseudocapacitance of rutile-like ruo2, Scientific Reports 7 (2017) 1–9. doi:10.1038/s41598-017-10331-z.
URL www.nature.com/scientificreports

[19] A. G. Kvashnin, D. G. Kvashnin, A. R. Oganov, Novel unexpected reconstructions of (100) and (111) surfaces of nacl: Theoretical prediction, Scientific Reports 9 (2019) 22–24. doi:10.1038/s41598-019-50548-8.
URL https://doi.org/10.1038/s41598-019-50548-8

[20] Y. Han, J. Wang, C. Ding, H. Gao, S. Pan, Q. Jia, J. Sun, Prediction of surface reconstructions using MAGUS, The Journal of Chemical Physics 158 (17) (2023) 174109. arXiv:https://pubs.aip.org/aip/jcp/article-pdf/doi/10.1063/5.0142281/17273365/174109_1_5.0142281.pdf, doi:10.1063/5.0142281.
URL https://doi.org/10.1063/5.0142281

[21] J. P. Perdew, K. Burke, M. Ernzerhof, Generalized gradient approximation made simple, Phys. Rev. Lett. 77 (1996) 3865–3868. doi:10.1103/PhysRevLett.77.3865.
URL http://link.aps.org/doi/10.1103/PhysRevLett.77.3865

[22] J. P. Perdew, A. Zunger, Self-interaction correction to density-functional approximations for many-electron systems, Phys. Rev. B 23 (1981) 5048–5079. doi:10.1103/PhysRevB.23.5048.
URL https://link.aps.org/doi/10.1103/PhysRevB.23.5048

[23] S. De Waele, K. Lejaeghere, M. Sluydts, S. Cottenier, Error estimates for density-functional theory predictions of surface energy and work function, Physical Review B 235418 (23) (2016) 1–13. doi:10.1103/PhysRevB.94.235418.

[24] A. Patra, J. E. Bates, J. Sun, J. P. Perdew, Properties of real metallic surfaces: Effects of density functional semilocality and van der waals nonlocality, Proceedings of the National Academy of Sciences 114 (44) (2017) E9188–E9196. arXiv:https://www.pnas.org/doi/pdf/10.1073/pnas.1713320114, doi:10.1073/pnas.1713320114.
URL https://www.pnas.org/doi/abs/10.1073/pnas.1713320114

[25] J. Sun, A. Ruzsinszky, J. P. Perdew, Strongly constrained and appropriately normed semilocal density functional, Phys. Rev. Lett. 115 (2015) 036402. doi:10.1103/PhysRevLett.115.036402.
URL https://link.aps.org/doi/10.1103/PhysRevLett.115.036402

[26] K. Mathew, J. H. Montoya, A. Faghaninia, S. Dwarakanath, M. Aykol, H. Tang, I. heng Chu, T. Smidt, B. Bocklund, M. Horton, J. Dagdelen, B. Wood, Z. K. Liu, J. Neaton, S. P. Ong, K. Persson, A. Jain, Atomate: A high-level interface to generate, execute, and analyze computational materials science workflows, Computational Materials Science 139 (2017) 140–152. doi:10.1016/j.commatsci.2017.07.030.
URL https://www.sciencedirect.com/science/article/pii/S0927025617303919

[27] P. Błoński, A. Kiejna, Structural, electronic, and magnetic properties of bcc iron surfaces, Surface Science 601 (1) (2007) 123–133. doi:https://doi.org/10.1016/j.susc.2006.09.013.
URL https://www.sciencedirect.com/science/article/pii/S0039602806009563

[28] D. C. Sorescu, Plane-wave dft investigations of the adsorption, diffusion, and activation of co on kinked fe(710) and fe(310) surfaces, The Journal of Physical Chemistry C 112 (28) (2008) 10472–10489. doi:10.1021/jp8008145.
URL https://doi.org/10.1021/jp8008145

[29] C.-F. Huo, B.-S. Wu, P. Gao, Y. Yang, Y.-W. Li, H. Jiao, The mechanism of potassium promoter: Enhancing the stability of active surfaces, Angewandte Chemie International Edition 50 (32) (2011) 7403–7406. arXiv:https://onlinelibrary.wiley.com/doi/pdf/10.1002/anie.201007484, doi:https://doi.org/10.1002/anie.201007484.
URL https://onlinelibrary.wiley.com/doi/abs/10.1002/anie.201007484

[30] J. G. Che, C. T. Chan, W.-E. Jian, T. C. Leung, Surface atomic structures, surface energies, and equilibrium crystal shape of molybdenum, Phys. Rev. B 57 (1998) 1875–1880. doi:10.1103/PhysRevB.57.1875.
URL https://link.aps.org/doi/10.1103/PhysRevB.57.1875

[31] T. Wang, X. Tian, Y. Yang, Y.-W. Li, J. Wang, M. Beller, H. Jiao, Structures of seven molybdenum surfaces and their coverage dependent hydrogen adsorption, Phys. Chem. Chem. Phys. 18 (2016) 6005–6012. doi:10.1039/C5CP07349A.
URL http://dx.doi.org/10.1039/C5CP07349A

[32] H. Lin, J.-X. Liu, H. Fan, W.-X. Li, Compensation between surface energy and hcp/fcc phase energy of late transition metals from first-principles calculations, The Journal of Physical Chemistry C 124 (20) (2020) 11005–11014. doi:10.1021/acs.jpcc.0c02142.
URL https://doi.org/10.1021/acs.jpcc.0c02142

[33] S. Schönecker, X. Li, B. Johansson, S. K. Kwon, L. Vitos, Thermal surface free energy and stress of iron, Scientific Reports 5 (2015) 14860. doi:10.1038/srep14860.
URL www.nature.com/scientificreports

[34] A. Price, H. Holl, A. Greenough, The surface energy and self diffusion coefficient of solid iron above 1350°c, Acta Metallurgica 12 (1) (1964) 49–58. doi:https://doi.org/10.1016/0001-6160(64)90053-7.
URL https://www.sciencedirect.com/science/article/pii/0001616064900537

[35] H. Ma, Y. Jiao, W. Guo, X. Liu, Y. Li, X.-D. Wen, Predicting crystal morphology using a geometric descriptor: A comparative study of elemental crystals with high-throughput dft calculations, The Journal of Physical Chemistry C 124 (29) (2020) 15920–15927. doi:10.1021/acs.jpcc.0c03537.
URL https://doi.org/10.1021/acs.jpcc.0c03537

[36] J. Sokolov, F. Jona, P. M. Marcus, Multilayer relaxation of a clean bcc fe111 surface, Phys. Rev. B 33 (1986) 1397–1400. doi:10.1103/PhysRevB.33.1397.
URL https://link.aps.org/doi/10.1103/PhysRevB.33.1397

[37] X. Sang, A. Kulovits, G. Wang, J. Wiezorek, High precision electronic charge density determination for l10-ordered $\gamma$-tial by quantitative convergent beam electron diffraction, Philosophical Magazine 92 (35) (2012) 4408–4424. doi:10.1080/14786435.2012.709324.
URL https://doi.org/10.1080/14786435.2012.709324

[38] P. Blaha, K. Schwarz, F. Tran, R. Laskowski, G. K. H. Madsen, L. D. Marks, WIEN2k: An APW+lo program for calculating the properties of solids, The Journal of Chemical Physics 152 (7) (2020) 074101. arXiv:https://pubs.aip.org/aip/jcp/article-pdf/doi/10.1063/1.5143061/16727313/074101_1_online.pdf, doi:10.1063/1.5143061.
URL https://doi.org/10.1063/1.5143061

[39] E. Bosoni, L. Beal, M. Bercx, P. Blaha, S. Blügel, J. Bröder, M. Callsen, S. Cottenier, A. Degomme, V. Dikan, K. Eimre, E. Flage-Larsen, M. Fornari, A. Garcia, L. Genovese, M. Giantomassi, S. P. Huber, H. Janssen, G. Kastlunger, M. Krack, G. Kresse, T. D. Kühne, K. Lejaeghere, G. K. H. Madsen, M. Marsman, N. Marzari, G. Michalicek, H. Mirhosseini, T. M. A. Müller, G. Petretto, C. J. Pickard, S. Poncé, G.-M. Rignanese, O. Rubel, T. Ruh, M. Sluydts, D. E. P. Vanpoucke, S. Vijay, M. Wolloch, D. Wortmann, A. V. Yakutovich, J. Yu, A. Zadoks, B. Zhu, G. Pizzi, How to verify the precision of density-functional-theory implementations via reproducible and universal workflows (2023). arXiv:2305.17274.

[40] Y. Song, J. Dai, R. Yang, Mechanism of oxygen adsorption on surfaces of $\gamma$-tial, Surface Science 606 (9) (2012) 852–857. doi:https://doi.org/10.1016/j.susc.2012.01.024.
URL https://www.sciencedirect.com/science/article/pii/S0039602812000404

[41] W. Setyawan, S. Curtarolo, High-throughput electronic band structure calculations: Challenges and tools, Computational Materials Science 49 (2) (2010) 299–312. doi:https://doi.org/10.1016/j.commatsci.2010.05.010.
URL https://www.sciencedirect.com/science/article/pii/S0927025610002697

Table 5: Detailed data for available surfaces in the database. We report materials project ID (mpid), sum formula (formula), Miller indices (hkl), slab thickness (thickness) in Å, top termination of the slab ($term_{top}$), bottom termination of the slab ($term_{bot}$), polarity (polar) and the surface energies of the top ($\gamma_{top}$) and bottom ($\gamma_{bot}$) surface in $J/m^2$.

| mpid | formula | hkl | thickness | $term_{top}$ | $term_{bot}$ | polar | $\gamma_{top}$ | $\gamma_{bot}$ |
|---|---|---|---|---|---|---|---|---|
| mp-1018028 | TiS | 001 | 11.26 | Ti | S | True | 2.32 | 2.09 |
| | | 100 | 12.26 | S | Ti | True | 1.58 | 1.47 |
| | | | 10.37 | Ti | S | True | 3.23 | 3.03 |
| | | 101 | 10.98 | Ti | S | True | 1.31 | 1.40 |
| | | | 10.27 | S | Ti | True | 2.46 | 2.78 |
| | | 102 | 10.72 | Ti | S | True | 1.74 | 1.67 |
| | | | 10.25 | S | Ti | True | 1.71 | 1.90 |
| | | 110 | 14.70 | TiS | TiS | False | 1.61 | 1.61 |
| | | 111 | 10.92 | Ti | S | True | 1.64 | 1.85 |
| | | 2-12 | 10.32 | TiS | TiS | False | 1.48 | 1.48 |
| | | 201 | 10.58 | S | Ti | True | 1.53 | 1.45 |
| | | | 10.14 | Ti | S | True | 2.19 | 2.03 |
| | | 221 | 10.69 | Ti | S | True | 1.65 | 1.73 |
| | | 3-10 | 11.05 | Ti | S | True | 1.60 | 1.66 |
| | | | 10.34 | S | Ti | True | 1.64 | 2.05 |
| | | 3-12 | 10.09 | S | Ti | True | 1.65 | 1.56 |
| | | | 10.39 | Ti | S | True | 1.58 | 1.71 |
| | | 302 | 10.58 | TiS | TiS | False | 1.47 | 1.44 |
| | | 332 | 10.32 | TiS | TiS | False | 1.71 | 1.71 |
| mp-102 | Co | 100 | 12.30 | Co | Co | False | 2.48 | 2.48 |
| | | 110 | 11.18 | Co | Co | False | 2.44 | 2.44 |
| | | 111 | 14.20 | Co | Co | False | 2.07 | 2.07 |
| | | 210 | 10.21 | Co | Co | False | 2.61 | 2.61 |
| | | 211 | 10.76 | Co | Co | False | 2.44 | 2.44 |
| | | 221 | 11.13 | Co | Co | False | 2.35 | 2.35 |
| | | 310 | 10.55 | Co | Co | False | 2.65 | 2.65 |
| | | 311 | 10.59 | Co | Co | False | 2.51 | 2.51 |
| | | 320 | 10.23 | Co | Co | False | 2.58 | 2.58 |
| | | 321 | 10.80 | Co | Co | False | 2.49 | 2.49 |
| | | 322 | 10.65 | Co | Co | False | 2.33 | 2.33 |
| | | 331 | 10.48 | Co | Co | False | 2.41 | 2.41 |
| | | 332 | 10.11 | Co | Co | False | 2.28 | 2.28 |
| mp-10905 | Al3Pt2 | 001 | 14.04 | Al | Al | False | 1.40 | 1.40 |
| | | | 14.70 | Al | Pt | False | 1.72 | 1.60 |
| | | | 14.60 | Pt | Al | False | 2.24 | 2.46 |
| | | 100 | 13.36 | Al | AlPt | False | 1.39 | 1.44 |
| | | | 13.36 | AlPt | AlPt | False | 1.80 | 1.80 |
| | | 101 | 10.44 | Al | Pt | False | 1.93 | 1.99 |

Continued on next page

Table 5: Detailed data for available surfaces in the database. We report materials project ID (mpid), sum formula (formula), Miller indices (hkl), slab thickness (thickness), top termination of the slab ($term_{top}$), bottom termination of the slab ($term_{bot}$), polarity (polar) and the surface energies of the top ($\gamma_{top}$) and bottom ($\gamma_{bot}$) surface in $J/m^2$.

| mpid | formula | hkl | thickness [Å] | $term_{top}$ | $term_{bot}$ | polar | $\gamma_{top}$ | $\gamma_{bot}$ |
|---|---|---|---|---|---|---|---|---|
| | | | 11.87 | Al | Al | False | 2.00 | 1.97 |
| | | 102 | 10.03 | Al | Al | False | 1.66 | 1.66 |
| | | | 10.49 | Pt | Al | False | 1.74 | 1.76 |
| | | | 11.89 | Al | Pt | False | 1.94 | 1.95 |
| | | 103 | 10.23 | Al | Al | False | 1.74 | 1.74 |
| | | | 10.77 | Pt | Al | False | 1.74 | 1.74 |
| | | | 10.67 | Al | Pt | False | 1.87 | 1.88 |
| | | 110 | 14.72 | Al3Pt2 | Al3Pt2 | False | 1.35 | 1.35 |
| | | 111 | 11.37 | Al | Pt | False | 1.56 | 1.54 |
| | | | 11.33 | Pt | Al | False | 1.71 | 1.75 |
| | | | 11.12 | Al | Al | False | 1.79 | 1.79 |
| | | 2-12 | 10.96 | Al | Al | False | 1.66 | 1.74 |
| | | | 11.37 | Al | Pt | False | 1.71 | 1.69 |
| | | | 10.76 | Pt | Pt | False | 1.82 | 1.82 |
| | | 2-13 | 10.61 | Al | Al | False | 1.77 | 1.71 |
| | | | 10.02 | Al | Pt | False | 1.75 | 1.78 |
| | | 201 | 10.06 | Pt | Al | False | 1.77 | 1.78 |
| | | | 11.39 | Al | Al | False | 1.83 | 1.83 |
| | | | 10.03 | Al | Pt | False | 1.94 | 1.98 |
| | | 203 | 11.08 | Al | Pt | False | 1.86 | 1.85 |
| | | | 11.00 | Pt | Al | False | 1.97 | 1.94 |
| | | | 11.02 | Al | Al | False | 1.95 | 1.95 |
| | | 221 | 10.14 | Al | Pt | False | 1.49 | 1.48 |
| | | | 10.12 | Pt | Al | False | 1.57 | 1.58 |
| | | | 10.01 | Al | Al | False | 1.60 | 1.60 |
| | | 223 | 10.34 | Al | Pt | False | 1.72 | 1.73 |
| | | | 10.73 | Al | Al | False | 1.74 | 1.72 |
| | | 3-10 | 10.56 | Al | AlPt | False | 1.42 | 1.44 |
| | | | 10.56 | AlPt | AlPt | False | 1.59 | 1.59 |
| | | 3-11 | 11.31 | Al | Pt | False | 1.68 | 1.70 |
| | | 3-13 | 10.66 | Pt | Al | False | 1.78 | 1.78 |
| | | | 10.29 | Al | Al | False | 1.80 | 1.80 |
| | | | 10.59 | Al | Pt | False | 1.87 | 1.95 |
| | | 301 | 10.45 | Al | Pt | False | 1.69 | 1.71 |
| | | | 10.42 | Pt | Al | False | 1.79 | 1.81 |
| | | | 10.30 | Al | Al | False | 1.80 | 1.80 |
| | | 302 | 10.68 | Al | AlPt | False | 1.84 | 1.87 |
| | | | 10.55 | AlPt | AlPt | False | 1.99 | 1.99 |

Continued on next page

Table 5: Detailed data for available surfaces in the database. We report materials project ID (mpid), sum formula (formula), Miller indices (hkl), slab thickness (thickness), top termination of the slab ($term_{top}$), bottom termination of the slab ($term_{bot}$), polarity (polar) and the surface energies of the top ($\gamma_{top}$) and bottom ($\gamma_{bot}$) surface in $J/m^2$.

| mpid | formula | hkl | thickness [Å] | $term_{top}$ | $term_{bot}$ | polar | $\gamma_{top}$ | $\gamma_{bot}$ |
|---|---|---|---|---|---|---|---|---|
| | | 310 | 10.78 | AlPt | AlPt | False | 1.45 | 1.45 |
| | | | 10.78 | Al | AlPt | False | 1.56 | 1.56 |
| | | 312 | 10.36 | Al3Pt2 | Al3Pt2 | False | 1.80 | 1.80 |
| | | 313 | 10.33 | Al | Pt | False | 1.79 | 1.81 |
| | | | 10.28 | Al | Al | False | 1.89 | 1.89 |
| | | | 10.27 | Pt | Al | False | 1.90 | 1.89 |
| | | 320 | 10.59 | Al | AlPt | False | 1.40 | 1.41 |
| | | | 10.59 | AlPt | AlPt | False | 1.50 | 1.50 |
| | | 323 | 10.46 | Pt | Al | False | 1.73 | 1.73 |
| | | | 10.20 | Al | Al | False | 1.75 | 1.75 |
| | | 331 | 10.31 | Al | Pt | False | 1.45 | 1.44 |
| | | | 10.29 | Pt | Al | False | 1.51 | 1.52 |
| | | | 10.22 | Al | Al | False | 1.53 | 1.53 |
| | | 332 | 10.63 | Al | AlPt | False | 1.60 | 1.60 |
| | | | 10.55 | AlPt | AlPt | False | 1.64 | 1.64 |
| mp-1138 | LiF | 100 | 14.29 | LiF | LiF | False | 0.32 | 0.32 |
| | | 110 | 10.11 | LiF | LiF | False | 0.77 | 0.77 |
| | | 210 | 10.04 | LiF | LiF | False | 0.55 | 0.55 |
| | | 211 | 10.84 | LiF | LiF | False | 1.08 | 1.08 |
| | | 221 | 10.21 | LiF | LiF | False | 0.93 | 0.93 |
| | | 310 | 10.98 | LiF | LiF | False | 0.47 | 0.47 |
| | | 320 | 10.76 | LiF | LiF | False | 0.63 | 0.63 |
| | | 321 | 10.37 | LiF | LiF | False | 0.84 | 0.84 |
| | | 322 | 10.40 | LiF | LiF | False | 0.95 | 0.95 |
| | | 332 | 10.01 | LiF | LiF | False | 1.07 | 1.07 |
| mp-11807 | LiPt | 100 | 10.31 | Li | Pt | False | 1.38 | 1.16 |
| | | | 11.10 | Pt | Li | False | 1.70 | 1.96 |
| | | 103 | 10.60 | Li | Pt | False | 1.36 | 1.41 |
| | | 110 | 10.99 | LiPt | LiPt | False | 1.38 | 1.38 |
| | | 111 | 11.09 | Pt | Li | False | 1.38 | 1.49 |
| | | 2-12 | 10.32 | LiPt | LiPt | False | 1.40 | 1.40 |
| | | 201 | 10.10 | Pt | Li | False | 1.46 | 1.61 |
| | | 302 | 10.37 | LiPt | LiPt | False | 1.29 | 1.25 |
| | | 332 | 10.28 | LiPt | LiPt | False | 1.46 | 1.46 |
| mp-12550 | AlCuPt2 | 001 | 12.21 | AlCu | Pt | True | 1.97 | 1.94 |
| | | 100 | 13.90 | AlPt | CuPt | True | 1.84 | 1.79 |
| | | 101 | 11.79 | AlPt | CuPt | True | 1.68 | 1.74 |
| | | 102 | 10.38 | AlPt | CuPt | True | 1.87 | 1.90 |

Continued on next page

Table 5: Detailed data for available surfaces in the database. We report materials project ID (mpid), sum formula (formula), Miller indices (hkl), slab thickness (thickness), top termination of the slab ($\text{term}_{\text{top}}$), bottom termination of the slab ($\text{term}_{\text{bot}}$), polarity (polar) and the surface energies of the top ($\gamma_{\text{top}}$) and bottom ($\gamma_{\text{bot}}$) surface in $J/m^2$.

| mpid | formula | hkl | thickness [Å] | $\text{term}_{\text{top}}$ | $\text{term}_{\text{bot}}$ | polar | $\gamma_{\text{top}}$ | $\gamma_{\text{bot}}$ |
|---|---|---|---|---|---|---|---|---|
| | | 103 | 10.60 | AlPt | CuPt | True | 1.90 | 1.93 |
| | | 110 | 12.64 | AlCu | Pt | True | 1.90 | 1.93 |
| | | 111 | 15.31 | AlCuPt2 | AlCuPt2 | False | 1.43 | 1.43 |
| | | 112 | 11.11 | AlCu | Pt | True | 1.70 | 1.75 |
| | | 113 | 10.74 | AlCuPt2 | AlCuPt2 | False | 1.81 | 1.81 |
| | | 201 | 11.22 | AlCu | Pt | True | 1.98 | 1.89 |
| | | 203 | 10.54 | AlCu | Pt | True | 1.85 | 1.86 |
| | | 210 | 11.54 | AlPt | CuPt | True | 1.91 | 1.97 |
| | | 211 | 10.29 | AlPt | CuPt | True | 1.73 | 1.73 |
| | | 212 | 10.58 | AlPt | CuPt | True | 1.61 | 1.63 |
| | | 213 | 10.22 | AlPt | CuPt | True | 1.73 | 1.76 |
| | | 221 | 11.07 | AlCu | Pt | True | 1.70 | 1.71 |
| | | 223 | 10.30 | AlCu | Pt | True | 1.58 | 1.65 |
| | | 301 | 10.52 | AlPt | CuPt | True | 1.91 | 1.93 |
| | | 302 | 10.02 | AlPt | CuPt | True | 1.88 | 1.88 |
| | | 310 | 10.67 | AlCu | Pt | True | 1.92 | 1.93 |
| | | 312 | 10.70 | AlCu | Pt | True | 1.78 | 1.78 |
| | | 313 | 10.24 | AlCuPt2 | AlCuPt2 | False | 1.67 | 1.67 |
| | | 320 | 10.46 | AlPt | CuPt | True | 1.96 | 1.97 |
| | | 321 | 11.03 | AlPt | CuPt | True | 1.80 | 1.85 |
| | | 323 | 10.80 | AlPt | CuPt | True | 1.56 | 1.57 |
| | | 331 | 10.85 | AlCuPt2 | AlCuPt2 | False | 1.78 | 1.78 |
| | | 332 | 10.31 | AlCu | Pt | True | 1.61 | 1.63 |
| mp-129 | Mo | 100 | 11.09 | Mo | Mo | False | 3.20 | 3.20 |
| | | 110 | 15.68 | Mo | Mo | False | 2.82 | 2.82 |
| | | 111 | 10.06 | Mo | Mo | False | 3.00 | 3.00 |
| | | 210 | 10.62 | Mo | Mo | False | 3.13 | 3.13 |
| | | 211 | 16.81 | Mo | Mo | False | 2.95 | 2.95 |
| | | 221 | 10.03 | Mo | Mo | False | 3.06 | 3.06 |
| | | 310 | 10.02 | Mo | Mo | False | 3.12 | 3.12 |
| | | 311 | 10.03 | Mo | Mo | False | 3.08 | 3.08 |
| | | 320 | 10.10 | Mo | Mo | False | 3.04 | 3.04 |
| | | 321 | 10.16 | Mo | Mo | False | 3.03 | 3.03 |
| | | 322 | 10.37 | Mo | Mo | False | 3.02 | 3.02 |
| | | 331 | 10.54 | Mo | Mo | False | 3.02 | 3.02 |
| | | 332 | 10.13 | Mo | Mo | False | 3.02 | 3.02 |
| mp-13 | Fe | 100 | 12.78 | Fe | Fe | False | 2.56 | 2.56 |
| | | 110 | 14.06 | Fe | Fe | False | 2.48 | 2.48 |

Continued on next page

Table 5: Detailed data for available surfaces in the database. We report materials project ID (mpid), sum formula (formula), Miller indices (hkl), slab thickness (thickness), top termination of the slab ($term_{top}$), bottom termination of the slab ($term_{bot}$), polarity (polar) and the surface energies of the top ($\gamma_{top}$) and bottom ($\gamma_{bot}$) surface in $J/m^2$.

| mpid | formula | hkl | thickness [Å] | $term_{top}$ | $term_{bot}$ | polar | $\gamma_{top}$ | $\gamma_{bot}$ |
|---|---|---|---|---|---|---|---|---|
| | | 111 | 10.66 | Fe | Fe | False | 2.75 | 2.75 |
| | | 210 | 10.80 | Fe | Fe | False | 2.60 | 2.60 |
| | | 211 | 10.44 | Fe | Fe | False | 2.63 | 2.63 |
| | | 221 | 10.89 | Fe | Fe | False | 2.69 | 2.69 |
| | | 310 | 11.68 | Fe | Fe | False | 2.59 | 2.59 |
| | | 311 | 10.70 | Fe | Fe | False | 2.68 | 2.68 |
| | | 320 | 10.63 | Fe | Fe | False | 2.59 | 2.59 |
| | | 321 | 10.63 | Fe | Fe | False | 2.66 | 2.66 |
| | | 322 | 10.68 | Fe | Fe | False | 2.71 | 2.71 |
| | | 331 | 10.10 | Fe | Fe | False | 2.67 | 2.67 |
| | | 332 | 10.29 | Fe | Fe | False | 2.69 | 2.69 |
| mp-13136 | WC | 100 | 15.35 | WC | WC | False | 0.72 | 0.72 |
| | | 110 | 10.85 | WC | WC | False | 1.98 | 1.98 |
| | | 210 | 10.79 | WC | WC | False | 1.11 | 1.11 |
| | | 211 | 11.64 | WC | WC | False | 1.76 | 1.76 |
| | | 221 | 10.96 | WC | WC | False | 2.07 | 2.07 |
| | | 310 | 10.40 | WC | WC | False | 0.91 | 0.91 |
| | | 320 | 10.34 | WC | WC | False | 1.42 | 1.42 |
| | | 321 | 11.13 | WC | WC | False | 1.63 | 1.63 |
| | | 322 | 10.10 | WC | WC | False | 2.02 | 2.02 |
| | | 332 | 10.75 | WC | WC | False | 2.25 | 2.25 |
| mp-135 | Li | 100 | 12.04 | Li | Li | False | 0.45 | 0.45 |
| | | 110 | 17.02 | Li | Li | False | 0.49 | 0.49 |
| | | 111 | 10.92 | Li | Li | False | 0.53 | 0.53 |
| | | 210 | 11.54 | Li | Li | False | 0.50 | 0.50 |
| | | 211 | 11.23 | Li | Li | False | 0.53 | 0.53 |
| | | 221 | 10.89 | Li | Li | False | 0.53 | 0.53 |
| | | 310 | 10.88 | Li | Li | False | 0.50 | 0.50 |
| | | 311 | 10.89 | Li | Li | False | 0.51 | 0.51 |
| | | 320 | 10.02 | Li | Li | False | 0.48 | 0.48 |
| | | 321 | 10.11 | Li | Li | False | 0.53 | 0.53 |
| | | 322 | 10.43 | Li | Li | False | 0.53 | 0.53 |
| | | 331 | 10.65 | Li | Li | False | 0.52 | 0.52 |
| | | 332 | 10.27 | Li | Li | False | 0.51 | 0.51 |
| mp-136 | Fe | 001 | 13.45 | Fe | Fe | False | 2.67 | 2.67 |
| | | 100 | 11.24 | Fe | Fe | False | 2.55 | 2.55 |
| | | | 11.95 | Fe | Fe | False | 3.08 | 3.08 |
| | | 101 | 11.40 | Fe | Fe | False | 2.90 | 2.90 |

Continued on next page

Table 5: Detailed data for available surfaces in the database. We report materials project ID (mpid), sum formula (formula), Miller indices (hkl), slab thickness (thickness), top termination of the slab ($term_{top}$), bottom termination of the slab ($term_{bot}$), polarity (polar) and the surface energies of the top ($\gamma_{top}$) and bottom ($\gamma_{bot}$) surface in $J/m^2$.

| mpid | formula | hkl | thickness [Å] | $term_{top}$ | $term_{bot}$ | polar | $\gamma_{top}$ | $\gamma_{bot}$ |
|---|---|---|---|---|---|---|---|---|
| | | | 10.78 | Fe | Fe | False | 3.25 | 3.25 |
| | | 102 | 10.89 | Fe | Fe | False | 2.83 | 2.83 |
| | | | 10.41 | Fe | Fe | False | 2.89 | 2.89 |
| | | 103 | 10.03 | Fe | Fe | False | 2.86 | 2.86 |
| | | | 10.76 | Fe | Fe | False | 2.88 | 2.88 |
| | | 110 | 10.95 | Fe | Fe | False | 2.70 | 2.70 |
| | | 111 | 11.02 | Fe | Fe | False | 2.91 | 2.91 |
| | | 2-12 | 10.28 | Fe | Fe | False | 2.90 | 2.90 |
| | | 2-13 | 10.15 | Fe | Fe | False | 3.01 | 3.01 |
| | | 201 | 10.33 | Fe | Fe | False | 2.92 | 2.92 |
| | | 203 | 10.72 | Fe | Fe | False | 2.83 | 2.83 |
| | | | 10.44 | Fe | Fe | False | 2.98 | 2.98 |
| | | 221 | 10.52 | Fe | Fe | False | 2.87 | 2.87 |
| | | 223 | 10.17 | Fe | Fe | False | 2.98 | 2.98 |
| | | 3-10 | 10.62 | Fe | Fe | False | 2.67 | 2.67 |
| | | | 10.09 | Fe | Fe | False | 2.80 | 2.80 |
| | | 3-11 | 10.27 | Fe | Fe | False | 2.88 | 2.88 |
| | | | 10.01 | Fe | Fe | False | 2.97 | 2.97 |
| | | 3-12 | 10.06 | Fe | Fe | False | 2.92 | 2.92 |
| | | | 10.55 | Fe | Fe | False | 2.94 | 2.94 |
| | | | 10.55 | Fe | Fe | False | 2.97 | 2.97 |
| | | 3-13 | 10.26 | Fe | Fe | False | 3.01 | 3.01 |
| | | | 10.04 | Fe | Fe | False | 3.12 | 3.12 |
| | | 301 | 10.02 | Fe | Fe | False | 2.83 | 2.83 |
| | | | 10.02 | Fe | Fe | False | 3.07 | 3.07 |
| | | 302 | 10.56 | Fe | Fe | False | 2.90 | 2.90 |
| | | 310 | 10.33 | Fe | Fe | False | 2.75 | 2.75 |
| | | | 10.13 | Fe | Fe | False | 2.82 | 2.82 |
| | | 313 | 10.02 | Fe | Fe | False | 2.95 | 2.95 |
| | | | 10.11 | Fe | Fe | False | 3.04 | 3.04 |
| | | 320 | 10.32 | Fe | Fe | False | 2.69 | 2.69 |
| | | 323 | 10.41 | Fe | Fe | False | 2.93 | 2.93 |
| | | 331 | 10.29 | Fe | Fe | False | 2.84 | 2.84 |
| | | 332 | 10.32 | Fe | Fe | False | 2.87 | 2.87 |
| mp-1487 | AlNi | 100 | 10.01 | Ni | Al | False | 2.23 | 2.30 |
| | | 110 | 14.15 | AlNi | AlNi | False | 1.51 | 1.51 |
| | | 111 | 10.73 | Ni | Al | False | 1.88 | 2.05 |
| | | 210 | 10.87 | Ni | Al | False | 1.91 | 1.91 |

Continued on next page

Table 5: Detailed data for available surfaces in the database. We report materials project ID (mpid), sum formula (formula), Miller indices (hkl), slab thickness (thickness), top termination of the slab ($term_{top}$), bottom termination of the slab ($term_{bot}$), polarity (polar) and the surface energies of the top ($\gamma_{top}$) and bottom ($\gamma_{bot}$) surface in $J/m^2$.

| mpid | formula | hkl | thickness [Å] | $term_{top}$ | $term_{bot}$ | polar | $\gamma_{top}$ | $\gamma_{bot}$ |
|---|---|---|---|---|---|---|---|---|
| | | 211 | 10.51 | AlNi | AlNi | False | 1.89 | 1.89 |
| | | 221 | 10.01 | Ni | Al | False | 1.81 | 1.89 |
| | | 310 | 10.85 | AlNi | AlNi | False | 2.04 | 2.04 |
| | | 311 | 10.78 | Al | Ni | False | 2.03 | 2.05 |
| | | 320 | 10.71 | Ni | Al | False | 1.78 | 1.77 |
| | | 321 | 10.70 | AlNi | AlNi | False | 1.77 | 1.77 |
| | | 322 | 10.06 | Al | Ni | False | 1.96 | 1.89 |
| | | 331 | 10.17 | Ni | Al | False | 1.72 | 1.79 |
| | | 332 | 10.36 | AlNi | AlNi | False | 1.91 | 1.91 |
| mp-1502 | Al2Pt | 100 | 16.22 | Al | Pt | False | 1.68 | 1.64 |
| | | 110 | 14.60 | Al2Pt | Al2Pt | False | 1.31 | 1.31 |
| | | 111 | 11.92 | Al | Al | False | 1.17 | 1.17 |
| | | | 12.77 | Pt | Al | False | 1.97 | 2.05 |
| | | | 12.77 | Pt | Al | False | 2.00 | 2.07 |
| | | 210 | 12.53 | Al | Pt | False | 1.56 | 1.55 |
| | | 211 | 10.84 | Al2Pt | Al2Pt | False | 1.49 | 1.49 |
| | | 221 | 11.31 | Pt | Al | False | 1.48 | 1.20 |
| | | 310 | 10.26 | Al2Pt | Al2Pt | False | 1.62 | 1.62 |
| | | 311 | 10.23 | Al | Pt | False | 1.53 | 1.55 |
| | | | 11.56 | Al | Al | False | 1.65 | 1.65 |
| | | 320 | 11.04 | Al | Pt | False | 1.48 | 1.48 |
| | | 321 | 10.25 | Al2Pt | Al2Pt | False | 1.36 | 1.36 |
| | | 322 | 11.09 | Al | Pt | False | 1.49 | 1.53 |
| | | 331 | 10.49 | Pt | Al | False | 1.60 | 1.25 |
| | | | 10.15 | Al | Al | False | 1.32 | 1.32 |
| | | 332 | 10.69 | Al2Pt | Al2Pt | False | 1.37 | 1.37 |
| mp-1539 | ZrTe | 001 | 13.53 | Zr | Te | True | 1.54 | 1.49 |
| | | 100 | 10.99 | Te | Zr | True | 1.14 | 1.12 |
| | | | 12.09 | Zr | Te | True | 2.12 | 2.13 |
| | | 101 | 10.45 | Zr | Te | True | 0.97 | 1.05 |
| | | | 12.13 | Te | Zr | True | 1.91 | 1.45 |
| | | 110 | 13.33 | ZrTe | ZrTe | False | 1.04 | 1.04 |
| | | 111 | 11.10 | Zr | Te | True | 0.92 | 1.40 |
| | | 2-12 | 12.21 | ZrTe | ZrTe | False | 1.11 | 1.11 |
| | | 201 | 10.87 | Te | Zr | True | 1.14 | 1.08 |
| | | | 10.36 | Zr | Te | True | 1.52 | 1.54 |
| | | 3-10 | 10.39 | Zr | Te | True | 1.11 | 1.10 |
| | | | 10.80 | Te | Zr | True | 1.44 | 1.24 |

Continued on next page

Table 5: Detailed data for available surfaces in the database. We report materials project ID (mpid), sum formula (formula), Miller indices (hkl), slab thickness (thickness), top termination of the slab ($term_{top}$), bottom termination of the slab ($term_{bot}$), polarity (polar) and the surface energies of the top ($\gamma_{top}$) and bottom ($\gamma_{bot}$) surface in $J/m^2$.

| mpid | formula | hkl | thickness [Å] | $term_{top}$ | $term_{bot}$ | polar | $\gamma_{top}$ | $\gamma_{bot}$ |
|---|---|---|---|---|---|---|---|---|
| | | 3-11 | 10.48 | Zr | Te | True | 0.37 | 1.36 |
| | | | 10.87 | Te | Zr | True | 1.25 | 1.17 |
| | | 3-12 | 10.82 | Te | Zr | True | 1.26 | 1.10 |
| | | 302 | 10.51 | ZrTe | ZrTe | False | 1.09 | 1.06 |
| | | 332 | 10.25 | ZrTe | ZrTe | False | 1.19 | 1.19 |
| mp-1894 | WC | 001 | 12.78 | W | C | True | 5.72 | 3.70 |
| | | 100 | 10.95 | W | C | True | 3.89 | 3.35 |
| | | | 11.79 | C | W | True | 6.61 | 7.39 |
| | | 101 | 11.64 | C | W | True | 3.76 | 3.80 |
| | | | 11.01 | W | C | True | 6.71 | 5.31 |
| | | 102 | 10.73 | C | W | True | 3.94 | 4.79 |
| | | | 10.31 | W | C | True | 4.89 | 4.25 |
| | | 110 | 10.21 | WC | WC | False | 3.77 | 3.77 |
| | | 111 | 11.03 | W | C | True | 4.37 | 4.13 |
| | | 2-12 | 10.17 | WC | WC | False | 3.99 | 3.99 |
| | | 201 | 10.58 | W | C | True | 3.80 | 3.49 |
| | | | 10.19 | C | W | True | 4.82 | 5.44 |
| | | 3-10 | 10.18 | W | C | True | 5.06 | 3.40 |
| | | | 10.82 | C | W | True | 3.73 | 3.93 |
| | | 3-11 | 10.71 | W | C | True | 4.30 | 3.83 |
| | | | 10.10 | C | W | True | 4.02 | 4.09 |
| | | 3-12 | 10.56 | W | C | True | 4.15 | 4.02 |
| | | | 10.03 | C | W | True | 4.03 | 4.25 |
| | | 302 | 10.14 | WC | WC | False | 3.81 | 3.66 |
| | | 332 | 10.12 | WC | WC | False | 4.10 | 4.10 |
| mp-1953 | TiAl | 001 | 18.30 | Al | Ti | False | 2.12 | 2.13 |
| | | 100 | 12.65 | Al | Ti | False | 2.02 | 2.00 |
| | | 101 | 20.81 | TiAl | TiAl | False | 1.69 | 1.69 |
| | | 102 | 10.71 | Al | Ti | False | 2.05 | 2.04 |
| | | 103 | 10.99 | TiAl | TiAl | False | 2.16 | 2.16 |
| | | 110 | 17.89 | TiAl | TiAl | False | 1.63 | 1.63 |
| | | 111 | 11.61 | Al | Ti | False | 2.07 | 2.05 |
| | | 112 | 11.37 | TiAl | TiAl | False | 2.03 | 2.03 |
| | | 113 | 10.64 | Al | Ti | False | 2.17 | 2.17 |
| | | 201 | 11.29 | Al | Ti | False | 1.90 | 1.88 |
| | | 203 | 10.24 | Al | Ti | False | 1.93 | 1.92 |
| | | 210 | 10.68 | Al | Ti | False | 1.95 | 1.92 |
| | | 211 | 10.81 | TiAl | TiAl | False | 1.88 | 1.88 |

Continued on next page

Table 5: Detailed data for available surfaces in the database. We report materials project ID (mpid), sum formula (formula), Miller indices (hkl), slab thickness (thickness), top termination of the slab ($term_{top}$), bottom termination of the slab ($term_{bot}$), polarity (polar) and the surface energies of the top ($\gamma_{top}$) and bottom ($\gamma_{bot}$) surface in $J/m^2$.

| mpid | formula | hkl | thickness [Å] | $term_{top}$ | $term_{bot}$ | polar | $\gamma_{top}$ | $\gamma_{bot}$ |
|---|---|---|---|---|---|---|---|---|
| | | 212 | 10.16 | Al | Ti | False | 1.99 | 1.98 |
| | | 213 | 10.14 | TiAl | TiAl | False | 1.95 | 1.95 |
| | | 221 | 10.14 | Al | Ti | False | 1.90 | 1.90 |
| | | 223 | 10.02 | Al | Ti | False | 2.08 | 2.06 |
| | | 301 | 10.04 | TiAl | TiAl | False | 1.92 | 1.92 |
| | | 302 | 10.64 | Al | Ti | False | 1.84 | 1.83 |
| | | 310 | 10.67 | TiAl | TiAl | False | 2.02 | 2.02 |
| | | 311 | 10.85 | Ti | Al | False | 1.95 | 1.98 |
| | | 312 | 10.59 | TiAl | TiAl | False | 1.84 | 1.84 |
| | | 313 | 10.03 | Al | Ti | False | 1.92 | 1.91 |
| | | 320 | 10.52 | Al | Ti | False | 1.85 | 1.83 |
| | | 321 | 10.72 | TiAl | TiAl | False | 1.83 | 1.83 |
| | | 322 | 10.55 | Al | Ti | False | 1.98 | 1.97 |
| | | 323 | 10.14 | TiAl | TiAl | False | 2.03 | 2.03 |
| | | 331 | 10.14 | Al | Ti | False | 1.82 | 1.82 |
| | | 332 | 10.08 | TiAl | TiAl | False | 1.96 | 1.96 |
| mp-2133 | ZnO | 001 | 13.91 | Zn | O2 | True | 1.64 | 1.48 |
| | | | 15.28 | O2 | Zn | True | 4.50 | 4.56 |
| | | 100 | 12.34 | ZnO | ZnO | False | 0.85 | 0.85 |
| | | | 10.44 | ZnO | ZnO | False | 2.28 | 2.28 |
| | | 101 | 12.13 | Zn | Zn | True | 1.33 | 1.57 |
| | | | 11.41 | O2 | Zn | True | 2.19 | 2.35 |
| | | | 11.41 | Zn | O2 | True | 2.36 | 2.19 |
| | | 102 | 11.18 | O2 | Zn | True | 1.74 | 1.79 |
| | | 110 | 11.51 | ZnO | ZnO | False | 0.89 | 0.89 |
| | | 2-12 | 10.85 | Zn | O2 | True | 2.45 | 2.46 |
| | | 201 | 10.38 | O2 | Zn | True | 1.54 | 1.60 |
| | | | 10.38 | Zn | O2 | True | 1.65 | 1.59 |
| | | 221 | 10.16 | Zn | O2 | True | 1.16 | 1.20 |
| | | | 10.47 | O2 | Zn | True | 1.31 | 1.36 |
| | | 3-10 | 10.05 | ZnO | ZnO | False | 0.89 | 0.89 |
| | | | 10.41 | ZnO | ZnO | False | 1.40 | 1.40 |
| | | 302 | 10.51 | Zn | O2 | True | 1.90 | 1.80 |
| | | 310 | 10.01 | ZnO | ZnO | False | 0.89 | 0.89 |
| | | 320 | 10.02 | ZnO | ZnO | False | 0.89 | 0.89 |
| | | | 10.24 | ZnO | ZnO | False | 1.20 | 1.20 |
| mp-219 | MoP | 001 | 11.14 | Mo | P | True | 2.58 | 2.94 |
| | | 100 | 12.14 | P | Mo | True | 2.28 | 1.92 |

Continued on next page

Table 5: Detailed data for available surfaces in the database. We report materials project ID (mpid), sum formula (formula), Miller indices (hkl), slab thickness (thickness), top termination of the slab ($\text{term}_{\text{top}}$), bottom termination of the slab ($\text{term}_{\text{bot}}$), polarity (polar) and the surface energies of the top ($\gamma_{\text{top}}$) and bottom ($\gamma_{\text{bot}}$) surface in $J/m^2$.

| mpid | formula | hkl | thickness [Å] | $\text{term}_{\text{top}}$ | $\text{term}_{\text{bot}}$ | polar | $\gamma_{\text{top}}$ | $\gamma_{\text{bot}}$ |
|---|---|---|---|---|---|---|---|---|
| | | | 10.27 | Mo | P | True | 3.66 | 3.99 |
| | | 101 | 10.86 | Mo | P | True | 1.85 | 2.02 |
| | | | 10.16 | P | Mo | True | 3.40 | 3.04 |
| | | 102 | 10.61 | Mo | P | True | 2.23 | 2.49 |
| | | | 10.15 | P | Mo | True | 2.48 | 2.45 |
| | | 103 | 10.09 | Mo | P | True | 2.47 | 2.54 |
| | | | 10.75 | P | Mo | True | 2.69 | 2.55 |
| | | 110 | 14.56 | MoP | MoP | False | 2.40 | 2.40 |
| | | 111 | 10.81 | Mo | P | True | 2.22 | 2.49 |
| | | 2-12 | 10.21 | MoP | MoP | False | 2.05 | 2.05 |
| | | 201 | 10.47 | P | Mo | True | 2.12 | 2.08 |
| | | | 10.04 | Mo | P | True | 2.82 | 2.94 |
| | | 3-10 | 10.94 | Mo | P | True | 2.28 | 2.42 |
| | | | 10.24 | P | Mo | True | 2.67 | 2.38 |
| | | 3-11 | 10.88 | P | Mo | True | 2.56 | 2.15 |
| | | | 10.21 | Mo | P | True | 2.34 | 2.32 |
| | | | 10.21 | P | Mo | True | 2.33 | 2.34 |
| | | 3-12 | 10.28 | Mo | P | True | 1.99 | 2.31 |
| | | | 10.87 | P | Mo | True | 2.25 | 2.19 |
| | | 3-13 | 10.62 | P | Mo | True | 2.07 | 2.00 |
| | | | 10.37 | Mo | P | True | 2.41 | 2.51 |
| | | 301 | 10.30 | Mo | P | True | 2.66 | 2.71 |
| | | 302 | 10.47 | MoP | MoP | False | 2.04 | 2.08 |
| | | 310 | 10.62 | Mo | P | True | 2.17 | 2.41 |
| | | | 10.36 | P | Mo | True | 2.45 | 2.39 |
| | | 332 | 10.21 | MoP | MoP | False | 2.37 | 2.37 |
| mp-2213 | FeNi | 001 | 12.53 | Fe | Ni | False | 2.44 | 2.41 |
| | | 100 | 11.30 | Fe | Ni | False | 2.40 | 2.46 |
| | | 101 | 14.38 | FeNi | FeNi | False | 2.14 | 2.14 |
| | | | 14.38 | FeNi | FeNi | False | 2.16 | 2.16 |
| | | 102 | 10.83 | Fe | Ni | False | 2.44 | 2.45 |
| | | 103 | 10.66 | FeNi | FeNi | False | 2.48 | 2.48 |
| | | 110 | 12.41 | FeNi | FeNi | False | 2.38 | 2.38 |
| | | 111 | 10.31 | Fe | Ni | False | 2.49 | 2.51 |
| | | 112 | 10.02 | FeNi | FeNi | False | 2.38 | 2.38 |
| | | 113 | 10.30 | Fe | Ni | False | 2.50 | 2.51 |
| | | 201 | 10.06 | Fe | Ni | False | 2.36 | 2.37 |
| | | 203 | 10.74 | Fe | Ni | False | 2.35 | 2.36 |

Continued on next page

Table 5: Detailed data for available surfaces in the database. We report materials project ID (mpid), sum formula (formula), Miller indices (hkl), slab thickness (thickness), top termination of the slab ($term_{top}$), bottom termination of the slab ($term_{bot}$), polarity (polar) and the surface energies of the top ($\gamma_{top}$) and bottom ($\gamma_{bot}$) surface in $J/m^2$.

| mpid | formula | hkl | thickness [Å] | $term_{top}$ | $term_{bot}$ | polar | $\gamma_{top}$ | $\gamma_{bot}$ |
|---|---|---|---|---|---|---|---|---|
| | | 210 | 10.65 | Fe | Ni | False | 2.51 | 2.57 |
| | | 211 | 10.71 | FeNi | FeNi | False | 2.46 | 2.46 |
| | | 212 | 10.90 | Fe | Ni | False | 2.45 | 2.46 |
| | | 213 | 10.56 | FeNi | FeNi | False | 2.38 | 2.38 |
| | | 221 | 10.75 | Fe | Ni | False | 2.52 | 2.52 |
| | | 223 | 10.28 | Fe | Ni | False | 2.47 | 2.48 |
| | | 301 | 10.59 | FeNi | FeNi | False | 2.41 | 2.41 |
| | | 302 | 10.21 | Fe | Ni | False | 2.30 | 2.31 |
| | | 310 | 10.30 | FeNi | FeNi | False | 2.54 | 2.54 |
| | | 311 | 10.45 | Fe | Ni | False | 2.50 | 2.53 |
| | | 312 | 10.14 | FeNi | FeNi | False | 2.42 | 2.42 |
| | | 313 | 10.21 | Fe | Ni | False | 2.40 | 2.40 |
| | | 320 | 10.08 | Fe | Ni | False | 2.47 | 2.52 |
| | | 321 | 10.25 | FeNi | FeNi | False | 2.49 | 2.49 |
| | | 322 | 10.05 | Ni | Fe | False | 2.52 | 2.52 |
| | | 323 | 10.19 | FeNi | FeNi | False | 2.50 | 2.50 |
| | | 331 | 10.22 | Fe | Ni | False | 2.47 | 2.48 |
| | | 332 | 10.11 | FeNi | FeNi | False | 2.52 | 2.52 |
| mp-2260 | FePt | 001 | 13.23 | Fe | Pt | True | 2.20 | 2.15 |
| | | 100 | 12.28 | Fe | Pt | True | 1.89 | 2.21 |
| | | 101 | 15.48 | FePt | FePt | False | 1.76 | 1.76 |
| | | 102 | 10.10 | Fe | Pt | True | 2.05 | 2.05 |
| | | 103 | 10.29 | FePt | FePt | False | 2.13 | 2.13 |
| | | 110 | 13.50 | FePt | FePt | False | 2.12 | 2.12 |
| | | 111 | 11.17 | Fe | Pt | True | 2.11 | 2.24 |
| | | 112 | 10.80 | FePt | FePt | False | 2.03 | 2.03 |
| | | 113 | 10.02 | Fe | Pt | True | 2.12 | 2.15 |
| | | 201 | 10.91 | Fe | Pt | True | 1.91 | 2.01 |
| | | 203 | 10.64 | Fe | Pt | True | 1.94 | 1.95 |
| | | 210 | 10.37 | Fe | Pt | True | 2.15 | 2.27 |
| | | 211 | 10.45 | FePt | FePt | False | 2.12 | 2.12 |
| | | 212 | 10.76 | Fe | Pt | True | 2.04 | 2.13 |
| | | 213 | 10.52 | FePt | FePt | False | 1.99 | 1.99 |
| | | 221 | 10.75 | Fe | Pt | True | 2.19 | 2.24 |
| | | 223 | 10.34 | Fe | Pt | True | 2.08 | 2.14 |
| | | 301 | 10.61 | FePt | FePt | False | 2.00 | 2.00 |
| | | 302 | 10.24 | Fe | Pt | True | 1.86 | 1.93 |
| | | 310 | 10.35 | FePt | FePt | False | 2.18 | 2.18 |

Continued on next page

Table 5: Detailed data for available surfaces in the database. We report materials project ID (mpid), sum formula (formula), Miller indices (hkl), slab thickness (thickness), top termination of the slab ($term_{top}$), bottom termination of the slab ($term_{bot}$), polarity (polar) and the surface energies of the top ($\gamma_{top}$) and bottom ($\gamma_{bot}$) surface in $J/m^2$.

| mpid | formula | hkl | thickness [Å] | $term_{top}$ | $term_{bot}$ | polar | $\gamma_{top}$ | $\gamma_{bot}$ |
|---|---|---|---|---|---|---|---|---|
| | | 311 | 10.51 | Fe | Pt | True | 2.11 | 2.19 |
| | | 312 | 10.20 | FePt | FePt | False | 2.05 | 2.05 |
| | | 313 | 10.32 | Fe | Pt | True | 1.99 | 2.04 |
| | | 320 | 10.21 | Fe | Pt | True | 2.16 | 2.24 |
| | | 321 | 10.39 | FePt | FePt | False | 2.17 | 2.17 |
| | | 322 | 10.19 | Pt | Fe | True | 2.20 | 2.15 |
| | | 323 | 10.38 | FePt | FePt | False | 2.14 | 2.14 |
| | | 331 | 10.46 | Fe | Pt | True | 2.18 | 2.21 |
| | | 332 | 10.35 | FePt | FePt | False | 2.21 | 2.21 |
| mp-22862 | NaCl | 100 | 19.56 | NaCl | NaCl | False | 0.11 | 0.11 |
| | | 110 | 13.83 | NaCl | NaCl | False | 0.30 | 0.30 |
| | | 210 | 11.25 | NaCl | NaCl | False | 0.23 | 0.23 |
| | | 211 | 10.27 | NaCl | NaCl | False | 0.49 | 0.49 |
| | | 221 | 10.24 | NaCl | NaCl | False | 0.51 | 0.51 |
| | | 310 | 11.49 | NaCl | NaCl | False | 0.20 | 0.20 |
| | | 320 | 10.07 | NaCl | NaCl | False | 0.26 | 0.26 |
| | | 321 | 11.20 | NaCl | NaCl | False | 0.38 | 0.38 |
| | | 322 | 10.16 | NaCl | NaCl | False | 0.56 | 0.56 |
| | | 332 | 10.13 | NaCl | NaCl | False | 0.49 | 0.49 |
| mp-23 | Ni | 100 | 12.16 | Ni | Ni | False | 2.16 | 2.16 |
| | | 110 | 11.06 | Ni | Ni | False | 2.24 | 2.24 |
| | | 111 | 14.04 | Ni | Ni | False | 1.85 | 1.85 |
| | | 210 | 10.10 | Ni | Ni | False | 2.37 | 2.37 |
| | | 211 | 10.64 | Ni | Ni | False | 2.19 | 2.19 |
| | | 221 | 11.00 | Ni | Ni | False | 2.12 | 2.12 |
| | | 310 | 10.44 | Ni | Ni | False | 2.36 | 2.36 |
| | | 311 | 10.48 | Ni | Ni | False | 2.26 | 2.26 |
| | | 320 | 10.12 | Ni | Ni | False | 2.36 | 2.36 |
| | | 321 | 10.68 | Ni | Ni | False | 2.28 | 2.28 |
| | | 322 | 10.54 | Ni | Ni | False | 2.09 | 2.09 |
| | | 331 | 10.36 | Ni | Ni | False | 2.19 | 2.19 |
| | | 332 | 10.00 | Ni | Ni | False | 2.06 | 2.06 |
| mp-23193 | KCl | 100 | 21.99 | KCl | KCl | False | 0.10 | 0.10 |
| | | 110 | 15.55 | KCl | KCl | False | 0.24 | 0.24 |
| | | 210 | 12.65 | KCl | KCl | False | 0.19 | 0.19 |
| | | 211 | 11.54 | KCl | KCl | False | 0.39 | 0.39 |
| | | 221 | 11.52 | KCl | KCl | False | 0.42 | 0.42 |
| | | 310 | 10.93 | KCl | KCl | False | 0.17 | 0.17 |

Continued on next page

Table 5: Detailed data for available surfaces in the database. We report materials project ID (mpid), sum formula (formula), Miller indices (hkl), slab thickness (thickness), top termination of the slab ($term_{top}$), bottom termination of the slab ($term_{bot}$), polarity (polar) and the surface energies of the top ($\gamma_{top}$) and bottom ($\gamma_{bot}$) surface in $J/m^2$.

| mpid | formula | hkl | thickness [Å] | $term_{top}$ | $term_{bot}$ | polar | $\gamma_{top}$ | $\gamma_{bot}$ |
|---|---|---|---|---|---|---|---|---|
| | | 320 | 11.33 | KCl | KCl | False | 0.21 | 0.21 |
| | | 321 | 10.92 | KCl | KCl | False | 0.31 | 0.31 |
| | | 322 | 11.43 | KCl | KCl | False | 0.36 | 0.36 |
| | | 332 | 10.05 | KCl | KCl | False | 0.52 | 0.52 |
| mp-2379 | CoSi2 | 100 | 14.61 | Si | Co | True | 2.27 | 2.23 |
| | | 110 | 13.15 | CoSi2 | CoSi2 | False | 1.67 | 1.67 |
| | | 111 | 10.74 | Si | Si | False | 1.46 | 1.46 |
| | | | 11.50 | Co | Si | True | 2.38 | 2.35 |
| | | 210 | 11.29 | Co | Si | True | 2.00 | 1.99 |
| | | 211 | 11.93 | CoSi2 | CoSi2 | False | 1.85 | 1.85 |
| | | 221 | 10.18 | Co | Si | True | 1.86 | 1.85 |
| | | 310 | 10.92 | CoSi2 | CoSi2 | False | 2.07 | 2.07 |
| | | 311 | 10.41 | Si | Si | False | 1.99 | 1.99 |
| | | 320 | 11.42 | Co | Si | True | 1.90 | 1.89 |
| | | 321 | 10.65 | CoSi2 | CoSi2 | False | 1.84 | 1.84 |
| | | 331 | 10.36 | Si | Si | False | 1.63 | 1.63 |
| | | 332 | 10.76 | CoSi2 | CoSi2 | False | 1.87 | 1.87 |
| mp-2744 | LiPd | 001 | 14.37 | Li | Pd | False | 1.25 | 1.25 |
| | | 100 | 10.42 | Pd | Li | False | 1.07 | 1.08 |
| | | | 11.22 | Li | Pd | False | 1.55 | 1.40 |
| | | 101 | 10.72 | Li | Pd | False | 1.04 | 1.01 |
| | | | 10.03 | Pd | Li | False | 1.21 | 1.43 |
| | | 102 | 11.45 | Pd | Li | False | 1.12 | 1.13 |
| | | | 10.41 | Li | Pd | False | 1.22 | 1.21 |
| | | 103 | 10.90 | Li | Pd | False | 1.13 | 1.21 |
| | | | 10.51 | Pd | Li | False | 1.22 | 1.17 |
| | | 110 | 12.49 | LiPd | LiPd | False | 1.07 | 1.07 |
| | | 111 | 11.18 | Li | Pd | False | 1.15 | 1.14 |
| | | 2-12 | 10.35 | LiPd | LiPd | False | 1.13 | 1.13 |
| | | 2-13 | 10.23 | Pd | Li | False | 1.16 | 1.18 |
| | | 201 | 10.58 | Pd | Li | False | 1.06 | 1.05 |
| | | | 10.19 | Li | Pd | False | 1.30 | 1.22 |
| | | 203 | 10.09 | Pd | Li | False | 1.11 | 1.10 |
| | | | 10.69 | Li | Pd | False | 1.16 | 1.14 |
| | | 221 | 10.61 | Li | Pd | False | 1.16 | 1.13 |
| | | 223 | 10.21 | Li | Pd | False | 1.15 | 1.15 |
| | | 3-10 | 10.30 | Li | Pd | False | 1.09 | 1.10 |
| | | | 10.60 | Pd | Li | False | 1.20 | 1.19 |

Continued on next page

Table 5: Detailed data for available surfaces in the database. We report materials project ID (mpid), sum formula (formula), Miller indices (hkl), slab thickness (thickness), top termination of the slab ($term_{top}$), bottom termination of the slab ($term_{bot}$), polarity (polar) and the surface energies of the top ($\gamma_{top}$) and bottom ($\gamma_{bot}$) surface in $J/m^2$.

| mpid | formula | hkl | thickness [Å] | $term_{top}$ | $term_{bot}$ | polar | $\gamma_{top}$ | $\gamma_{bot}$ |
|---|---|---|---|---|---|---|---|---|
| | | 3-11 | 10.80 | Li | Pd | False | 1.13 | 1.11 |
| | | | 10.50 | Pd | Li | False | 1.15 | 1.22 |
| | | 3-12 | 10.25 | Li | Pd | False | 1.13 | 1.11 |
| | | | 10.53 | Pd | Li | False | 1.12 | 1.13 |
| | | 3-13 | 10.47 | Li | Pd | False | 1.06 | 1.16 |
| | | | 10.73 | Pd | Li | False | 1.10 | 1.11 |
| | | 301 | 10.62 | Pd | Li | False | 1.00 | 1.07 |
| | | | 10.62 | Li | Pd | False | 1.21 | 1.17 |
| | | 302 | 10.45 | LiPd | LiPd | False | 1.05 | 1.04 |
| | | 310 | 10.45 | Li | Pd | False | 1.11 | 1.12 |
| | | | 10.22 | Pd | Li | False | 1.17 | 1.16 |
| | | 311 | 10.42 | Li | Pd | False | 1.19 | 1.18 |
| | | 313 | 10.29 | Pd | Li | False | 1.08 | 1.09 |
| | | 320 | 10.11 | Li | Pd | False | 1.09 | 1.09 |
| | | | 10.30 | Pd | Li | False | 1.15 | 1.15 |
| | | 323 | 10.23 | Li | Pd | False | 1.14 | 1.15 |
| | | | 10.15 | Pd | Li | False | 1.15 | 1.16 |
| | | 331 | 10.35 | Li | Pd | False | 1.14 | 1.12 |
| | | 332 | 10.38 | LiPd | LiPd | False | 1.15 | 1.15 |
| mp-2746 | MoC | 100 | 15.34 | MoC | MoC | False | 0.85 | 0.85 |
| | | 110 | 10.85 | MoC | MoC | False | 1.99 | 1.99 |
| | | 210 | 10.78 | MoC | MoC | False | 1.10 | 1.10 |
| | | 211 | 11.63 | MoC | MoC | False | 1.88 | 1.88 |
| | | 221 | 10.96 | MoC | MoC | False | 2.10 | 2.10 |
| | | 310 | 10.40 | MoC | MoC | False | 0.92 | 0.92 |
| | | 320 | 10.33 | MoC | MoC | False | 1.40 | 1.40 |
| | | 321 | 11.13 | MoC | MoC | False | 1.65 | 1.65 |
| | | 322 | 10.10 | MoC | MoC | False | 2.19 | 2.19 |
| | | 332 | 10.75 | MoC | MoC | False | 2.31 | 2.31 |
| mp-284 | AlCo | 100 | 12.69 | Al | Co | False | 2.80 | 2.79 |
| | | 110 | 13.96 | AlCo | AlCo | False | 2.04 | 2.04 |
| | | 111 | 10.58 | Al | Co | False | 2.62 | 2.63 |
| | | 210 | 10.72 | Al | Co | False | 2.44 | 2.48 |
| | | 211 | 10.36 | AlCo | AlCo | False | 2.47 | 2.47 |
| | | 221 | 10.81 | Al | Co | False | 2.46 | 2.51 |
| | | 310 | 10.70 | AlCo | AlCo | False | 2.53 | 2.53 |
| | | 311 | 10.63 | Co | Al | False | 2.58 | 2.60 |
| | | 320 | 10.56 | Al | Co | False | 2.31 | 2.35 |

Continued on next page

Table 5: Detailed data for available surfaces in the database. We report materials project ID (mpid), sum formula (formula), Miller indices (hkl), slab thickness (thickness), top termination of the slab ($term_{top}$), bottom termination of the slab ($term_{bot}$), polarity (polar) and the surface energies of the top ($\gamma_{top}$) and bottom ($\gamma_{bot}$) surface in $J/m^2$.

| mpid | formula | hkl | thickness [Å] | $term_{top}$ | $term_{bot}$ | polar | $\gamma_{top}$ | $\gamma_{bot}$ |
|---|---|---|---|---|---|---|---|---|
| | | 321 | 10.55 | AlCo | AlCo | False | 2.41 | 2.41 |
| | | 322 | 10.60 | Co | Al | False | 2.57 | 2.53 |
| | | 331 | 10.03 | Al | Co | False | 2.38 | 2.41 |
| | | 332 | 10.22 | AlCo | AlCo | False | 2.55 | 2.55 |
| mp-463 | KF | 100 | 18.58 | KF | KF | False | 0.13 | 0.13 |
| | | 110 | 13.14 | KF | KF | False | 0.37 | 0.37 |
| | | 210 | 10.68 | KF | KF | False | 0.27 | 0.27 |
| | | 211 | 11.92 | KF | KF | False | 0.59 | 0.59 |
| | | 221 | 11.50 | KF | KF | False | 0.63 | 0.63 |
| | | 310 | 10.91 | KF | KF | False | 0.24 | 0.24 |
| | | 320 | 11.04 | KF | KF | False | 0.31 | 0.31 |
| | | 321 | 10.64 | KF | KF | False | 0.47 | 0.47 |
| | | 322 | 10.94 | KF | KF | False | 0.54 | 0.54 |
| | | 332 | 10.75 | KF | KF | False | 0.59 | 0.59 |
| mp-492 | TiN | 100 | 14.89 | TiN | TiN | False | 1.24 | 1.24 |
| | | 110 | 10.53 | TiN | TiN | False | 2.62 | 2.62 |
| | | 111 | 11.05 | N2 | Ti | True | 2.05 | 4.66 |
| | | 210 | 10.46 | TiN | TiN | False | 1.95 | 1.95 |
| | | 211 | 11.29 | TiN | TiN | False | 2.73 | 2.73 |
| | | 221 | 10.63 | TiN | TiN | False | 2.90 | 2.90 |
| | | 310 | 10.09 | TiN | TiN | False | 1.73 | 1.73 |
| | | 311 | 10.90 | Ti | N2 | True | 2.72 | 2.09 |
| | | 320 | 10.03 | TiN | TiN | False | 2.22 | 2.22 |
| | | 321 | 10.80 | TiN | TiN | False | 2.65 | 2.65 |
| | | 322 | 10.83 | TiN | TiN | False | 2.99 | 2.99 |
| | | 331 | 10.25 | N2 | Ti | True | 2.39 | 3.17 |
| | | 332 | 10.43 | TiN | TiN | False | 3.04 | 3.04 |
| mp-522 | CuAu | 001 | 12.82 | Au | Cu | True | 1.15 | 1.14 |
| | | 100 | 10.02 | Au | Cu | True | 1.23 | 1.07 |
| | | 101 | 15.79 | CuAu | CuAu | False | 0.90 | 0.90 |
| | | 102 | 10.03 | Au | Cu | True | 1.13 | 1.09 |
| | | 103 | 10.11 | CuAu | CuAu | False | 1.13 | 1.13 |
| | | 110 | 14.18 | CuAu | CuAu | False | 1.09 | 1.09 |
| | | 111 | 11.52 | Au | Cu | True | 1.21 | 1.13 |
| | | 112 | 10.87 | CuAu | CuAu | False | 1.11 | 1.11 |
| | | 201 | 10.00 | Au | Cu | True | 1.10 | 1.01 |
| | | 210 | 10.89 | Au | Cu | True | 1.23 | 1.15 |
| | | 211 | 10.88 | CuAu | CuAu | False | 1.09 | 1.09 |

Continued on next page

Table 5: Detailed data for available surfaces in the database. We report materials project ID (mpid), sum formula (formula), Miller indices (hkl), slab thickness (thickness), top termination of the slab ($term_{top}$), bottom termination of the slab ($term_{bot}$), polarity (polar) and the surface energies of the top ($\gamma_{top}$) and bottom ($\gamma_{bot}$) surface in $J/m^2$.

| mpid | formula | hkl | thickness [Å] | $term_{top}$ | $term_{bot}$ | polar | $\gamma_{top}$ | $\gamma_{bot}$ |
|---|---|---|---|---|---|---|---|---|
| | | 212 | 11.02 | Au | Cu | True | 1.13 | 1.08 |
| | | 213 | 10.60 | CuAu | CuAu | False | 1.07 | 1.07 |
| | | 221 | 10.25 | Au | Cu | True | 1.17 | 1.13 |
| | | 301 | 10.16 | CuAu | CuAu | False | 1.06 | 1.06 |
| | | 310 | 10.87 | CuAu | CuAu | False | 1.18 | 1.18 |
| | | 312 | 10.55 | CuAu | CuAu | False | 1.07 | 1.07 |
| | | 321 | 10.09 | CuAu | CuAu | False | 1.12 | 1.12 |
| | | 323 | 10.65 | CuAu | CuAu | False | 1.15 | 1.15 |
| | | 332 | 10.13 | CuAu | CuAu | False | 1.17 | 1.17 |
| mp-579 | CrC | 100 | 14.38 | CrC | CrC | False | 1.02 | 1.02 |
| | | 110 | 10.17 | CrC | CrC | False | 2.22 | 2.22 |
| | | 210 | 10.10 | CrC | CrC | False | 1.33 | 1.33 |
| | | 211 | 10.90 | CrC | CrC | False | 2.32 | 2.32 |
| | | 221 | 10.27 | CrC | CrC | False | 2.58 | 2.58 |
| | | 310 | 11.04 | CrC | CrC | False | 0.99 | 0.99 |
| | | 320 | 10.82 | CrC | CrC | False | 1.64 | 1.64 |
| | | 321 | 10.43 | CrC | CrC | False | 2.07 | 2.07 |
| | | 322 | 10.46 | CrC | CrC | False | 2.69 | 2.69 |
| | | 332 | 10.07 | CrC | CrC | False | 2.78 | 2.78 |
| mp-631 | TiC | 100 | 15.16 | TiC | TiC | False | 1.61 | 1.61 |
| | | 110 | 10.72 | TiC | TiC | False | 3.61 | 3.61 |
| | | 210 | 10.65 | TiC | TiC | False | 2.63 | 2.63 |
| | | 211 | 11.49 | TiC | TiC | False | 4.08 | 4.08 |
| | | 221 | 10.83 | TiC | TiC | False | 4.33 | 4.33 |
| | | 310 | 10.27 | TiC | TiC | False | 2.39 | 2.39 |
| | | 320 | 10.21 | TiC | TiC | False | 3.02 | 3.02 |
| | | 321 | 11.00 | TiC | TiC | False | 3.67 | 3.67 |
| | | 322 | 11.03 | TiC | TiC | False | 4.67 | 4.67 |
| | | 332 | 10.62 | TiC | TiC | False | 4.82 | 4.82 |
| mp-66 | C | 100 | 13.40 | C | C | False | 8.42 | 8.42 |
| | | 110 | 11.37 | C | C | False | 5.14 | 5.14 |
| | | 111 | 10.83 | C | C | False | 5.07 | 5.07 |
| | | | 11.86 | C | C | False | 12.28 | 12.28 |
| | | 210 | 10.79 | C | C | False | 5.68 | 5.68 |
| | | 211 | 10.94 | C | C | False | 5.75 | 5.75 |
| | | 221 | 10.42 | C | C | False | 4.80 | 4.80 |
| | | | 10.42 | C | C | False | 7.45 | 7.45 |
| | | 310 | 10.74 | C | C | False | 6.80 | 6.80 |

Continued on next page

Table 5: Detailed data for available surfaces in the database. We report materials project ID (mpid), sum formula (formula), Miller indices (hkl), slab thickness (thickness), top termination of the slab ($term_{top}$), bottom termination of the slab ($term_{bot}$), polarity (polar) and the surface energies of the top ($\gamma_{top}$) and bottom ($\gamma_{bot}$) surface in $J/m^2$.

| mpid | formula | hkl | thickness [Å] | $term_{top}$ | $term_{bot}$ | polar | $\gamma_{top}$ | $\gamma_{bot}$ |
|---|---|---|---|---|---|---|---|---|
| | | 311 | 11.04 | C | C | False | 5.93 | 5.93 |
| | | | 10.51 | C | C | False | 6.51 | 6.51 |
| | | 320 | 10.66 | C | C | False | 5.55 | 5.55 |
| | | 321 | 10.03 | C | C | False | 5.69 | 5.69 |
| | | 322 | 10.18 | C | C | False | 5.51 | 5.51 |
| | | | 10.18 | C | C | False | 5.54 | 5.54 |
| | | 331 | 10.04 | C | C | False | 4.64 | 4.64 |
| | | | 10.45 | C | C | False | 8.57 | 8.57 |
| | | 332 | 10.29 | C | C | False | 6.57 | 6.57 |
| mp-91 | W | 100 | 11.10 | W | W | False | 4.01 | 4.01 |
| | | 110 | 15.69 | W | W | False | 3.23 | 3.23 |
| | | 111 | 10.07 | W | W | False | 3.53 | 3.53 |
| | | 210 | 10.63 | W | W | False | 3.73 | 3.73 |
| | | 211 | 10.35 | W | W | False | 3.47 | 3.47 |
| | | 221 | 10.04 | W | W | False | 3.60 | 3.60 |
| | | 310 | 10.03 | W | W | False | 3.77 | 3.77 |
| | | 311 | 10.04 | W | W | False | 3.69 | 3.69 |
| | | 320 | 10.11 | W | W | False | 3.59 | 3.59 |
| | | 321 | 10.17 | W | W | False | 3.53 | 3.53 |
| | | 322 | 10.38 | W | W | False | 3.58 | 3.58 |
| | | 331 | 10.55 | W | W | False | 3.52 | 3.52 |
| | | 332 | 10.14 | W | W | False | 3.59 | 3.59 |
| mp-930 | ZrP | 100 | 18.52 | ZrP | ZrP | False | 0.70 | 0.70 |
| | | 110 | 13.10 | ZrP | ZrP | False | 1.42 | 1.42 |
| | | 210 | 10.65 | ZrP | ZrP | False | 1.18 | 1.18 |
| | | 211 | 11.88 | ZrP | ZrP | False | 1.74 | 1.74 |
| | | 221 | 11.47 | ZrP | ZrP | False | 1.84 | 1.84 |
| | | 310 | 10.88 | ZrP | ZrP | False | 1.04 | 1.04 |
| | | 320 | 11.01 | ZrP | ZrP | False | 1.28 | 1.28 |
| | | 321 | 10.61 | ZrP | ZrP | False | 1.65 | 1.65 |
| | | 322 | 10.91 | ZrP | ZrP | False | 1.93 | 1.93 |
| | | 332 | 10.72 | ZrP | ZrP | False | 1.95 | 1.95 |
| mp-987 | ZnCu | 100 | 10.36 | Cu | Zn | False | 1.33 | 1.36 |
| | | 110 | 14.65 | ZnCu | ZnCu | False | 1.09 | 1.09 |
| | | 111 | 11.11 | Cu | Zn | False | 1.27 | 1.41 |
| | | 210 | 11.25 | Cu | Zn | False | 1.26 | 1.28 |
| | | 211 | 10.88 | ZnCu | ZnCu | False | 1.05 | 1.05 |
| | | 221 | 10.36 | Cu | Zn | False | 1.21 | 1.27 |

Continued on next page

Table 5: Detailed data for available surfaces in the database. We report materials project ID (mpid), sum formula (formula), Miller indices (hkl), slab thickness (thickness), top termination of the slab ($\text{term}_{\text{top}}$), bottom termination of the slab ($\text{term}_{\text{bot}}$), polarity (polar) and the surface energies of the top ($\gamma_{\text{top}}$) and bottom ($\gamma_{\text{bot}}$) surface in $J/m^2$.

| mpid | formula | hkl | thickness [Å] | $\text{term}_{\text{top}}$ | $\text{term}_{\text{bot}}$ | polar | $\gamma_{\text{top}}$ | $\gamma_{\text{bot}}$ |
|---|---|---|---|---|---|---|---|---|
| | | 310 | 10.30 | ZnCu | ZnCu | False | 1.30 | 1.30 |
| | | 311 | 10.27 | Zn | Cu | False | 1.32 | 1.33 |
| | | 320 | 10.26 | Cu | Zn | False | 1.22 | 1.23 |
| | | 321 | 10.29 | ZnCu | ZnCu | False | 1.14 | 1.14 |
| | | 322 | 10.41 | Zn | Cu | False | 1.31 | 1.26 |
| | | 331 | 10.53 | Cu | Zn | False | 1.19 | 1.23 |
| | | 332 | 10.10 | ZnCu | ZnCu | False | 1.31 | 1.31 |
